# Supplementary material for: Allowed $\beta^-$ decay of bare atoms with A$\sim$ 60-80 in stellar environments
Source: arXiv:2304.00834 source file (2023-09-03)
Supplement: Supplementary file 1 [file Supplemental_Material.pdf]

## Supplemental Material: Allowed $\beta^-$ Decay of Bare Atoms ( $A \sim 60-80$ ) in Stellar Environments

Arkabrata Gupta,<sup>1</sup> Chirashree Lahiri,<sup>2</sup> and S. Sarkar<sup>1,\*</sup>

<sup>1</sup>*Department of Physics, Indian Institute of Engineering Science and Technology, Shibpur, Howrah-711103, India*

<sup>2</sup>*Department of Physics, Surendranath Evening College, 24/2 M. G. Road, Kolkata- 700009, India*

In the main manuscript we have shown the data (Table IV.A, Table IV.B, Table V, Table VI.A, Table VI.B) only for those excited levels which have contribution  $> 0.1\%$ , with respect to total decay rate. However, in Table VII we have given total decay rate taking into account all of the transitions. The remaining data are presented in this supplemental material.

### I. $\beta^-$ DECAY RATES: REST OF THE DATA

In this section we have tabulated the data for  $^{65}\text{Ni}$ ,  $^{66}\text{Cu}$ ,  $^{75}\text{Ge}$ ,  $^{81}\text{Se}$ .

Table (I.A) : This table corresponds to Table (IV.A) of the main manuscript.

Table (I.B) : This table corresponds to Table (IV.B) of the main manuscript.

Table (II) : This table corresponds to Table (V) of the main manuscript.

Table (III.A) : This table corresponds to Table (VI.A) of the main manuscript.

Table (III.B) : This table corresponds to Table (VI.B) of the main manuscript.

### II. $\beta^-$ DECAY RATES WITH MOMENTUM INDEPENDENT LEPTON PHASE SPACE FACTOR

Certain combinations of electron radial wave functions evaluated at nuclear radius  $R$  (in the unit of  $\hbar/m_e c$ ) were first introduced by Konopinski and Uhlenbeck [1] as  $L_k$ 's. The value for  $k = 0$  can be approximated as

$$L_0 = \frac{1 + \sqrt{1 - \alpha^2 Z^2}}{2}. \quad (1)$$

Here,  $\alpha$  is the fine structure constant. In the work of Behrens and Jänecke [2], the authors had taken a different form of  $L_0$ , which includes a slight dependence on the momentum. In the main manuscript, we have used momentum dependent phase space factor as given by Wilkinson [3]. However, we have also calculated the phase space factor in  $L_0$  approximation given in Eq.1. We have found that, inclusion of the momentum dependence in phase space factor, changes the continuum decay rate 1% - 2% only.

In this section, neutral atom half-life, and bare atom total decay rate with half-life for different temperature density combinations, calculated with momentum independent phase space factor has been presented.

Table (IV) : This table corresponds to Table (I) of the main manuscript.

Table (V) : This table corresponds to Table (VII) of the main manuscript.

- 
- [1] E. J. Konopinski and G. E. Uhlenbeck, Phys. Rev. **60**, 308 (1941).  
 [2] H. Behrens and J. Jänecke, Numerical Tables for Beta-Decay and Electron Capture, Springer (1969).  
 [3] D. H. Wilkinson, Nuclear Instruments and Methods in Physics Research A **290**, 509 (1990).  
 [4] National Nuclear Data Center,

- (<https://www.nndc.bnl.gov/>).  
 [5] K. Takahashi and K. Yokoi, Nucl. Phys. A **404**, 578 (1983).  
 [6] K. Cosner and, J. W. Truran, Astrophysics and Space Science **78**, 85 (1981).

TABLE (I.A) Bound state decay rate ( $\lambda_b$  in  $sec^{-1}$ ) and continuum state decay rate ( $\lambda_c$  in  $sec^{-1}$ ) variation with temperature at a free electron density  $n_e = 1 \times 10^{27}/cm^3$  for each transition. There are blank spaces in column 4 and column 5 because those excited states are not populated at the corresponding temperature.

| Transition Details            |           |           | $n_e = 1 \times 10^{27}/cm^3$ |                        |                        |                        |
|-------------------------------|-----------|-----------|-------------------------------|------------------------|------------------------|------------------------|
| <i>Decay</i>                  | $J_p^\pi$ | $J_d^\pi$ | T = $1 \times 10^8$ K         |                        | T = $5 \times 10^8$ K  |                        |
|                               |           |           | $\lambda_c$                   | $\lambda_b$            | $\lambda_c$            | $\lambda_b$            |
| $^{65}Ni \rightarrow ^{65}Cu$ | $5/2_1^-$ | $3/2_1^-$ | $4.50 \times 10^{-5}$         | $2.71 \times 10^{-7}$  | $4.51 \times 10^{-5}$  | $2.72 \times 10^{-7}$  |
|                               |           | $5/2_1^-$ | $3.58 \times 10^{-6}$         | $9.57 \times 10^{-8}$  | $3.59 \times 10^{-6}$  | $9.58 \times 10^{-8}$  |
|                               |           | $7/2_1^-$ | $2.02 \times 10^{-5}$         | $1.18 \times 10^{-6}$  | $2.04 \times 10^{-5}$  | $1.18 \times 10^{-6}$  |
|                               |           | $5/2_2^-$ | $1.78 \times 10^{-6}$         | $1.53 \times 10^{-7}$  | $1.80 \times 10^{-6}$  | $1.54 \times 10^{-7}$  |
|                               |           | $3/2_2^-$ | $1.42 \times 10^{-7}$         | $1.72 \times 10^{-8}$  | $1.44 \times 10^{-7}$  | $1.73 \times 10^{-8}$  |
|                               |           | $7/2_2^-$ | $2.38 \times 10^{-9}$         | $7.90 \times 10^{-9}$  | $2.75 \times 10^{-9}$  | $8.19 \times 10^{-9}$  |
|                               |           | $5/2_3^-$ | $1.21 \times 10^{-12}$        | $8.00 \times 10^{-12}$ | $1.49 \times 10^{-12}$ | $8.41 \times 10^{-12}$ |
|                               | $1/2_1^-$ | $3/2_1^-$ | $5.39 \times 10^{-3}$         | $3.05 \times 10^{-5}$  | $5.40 \times 10^{-3}$  | $3.05 \times 10^{-5}$  |
|                               |           | $1/2_1^-$ | $2.38 \times 10^{-5}$         | $3.33 \times 10^{-7}$  | $2.38 \times 10^{-5}$  | $3.33 \times 10^{-7}$  |
|                               |           | $3/2_2^-$ | $3.10 \times 10^{-7}$         | $3.01 \times 10^{-8}$  | $3.13 \times 10^{-7}$  | $3.02 \times 10^{-8}$  |
|                               | $3/2_1^-$ | $3/2_1^-$ |                               |                        | $8.58 \times 10^{-4}$  | $3.82 \times 10^{-6}$  |
|                               |           | $1/2_1^-$ |                               |                        | $4.41 \times 10^{-6}$  | $4.46 \times 10^{-8}$  |
|                               |           | $5/2_1^-$ |                               |                        | $2.14 \times 10^{-5}$  | $3.46 \times 10^{-7}$  |
|                               |           | $5/2_2^-$ |                               |                        | $1.45 \times 10^{-6}$  | $5.70 \times 10^{-8}$  |
|                               |           | $3/2_2^-$ |                               |                        | $1.07 \times 10^{-8}$  | $5.27 \times 10^{-10}$ |
|                               |           | $5/2_3^-$ |                               |                        | $4.01 \times 10^{-7}$  | $6.39 \times 10^{-8}$  |
|                               |           | $1/2_2^-$ |                               |                        | $3.57 \times 10^{-8}$  | $9.59 \times 10^{-9}$  |
|                               |           | $3/2_3^-$ |                               |                        | $8.99 \times 10^{-10}$ | $6.11 \times 10^{-10}$ |
|                               | $1_1^+$   | $0_1^+$   | $1.19 \times 10^{-3}$         | $4.85 \times 10^{-6}$  | $1.19 \times 10^{-3}$  | $4.85 \times 10^{-6}$  |
|                               |           | $2_1^+$   | $3.48 \times 10^{-4}$         | $4.21 \times 10^{-6}$  | $3.49 \times 10^{-4}$  | $4.21 \times 10^{-6}$  |
|                               |           | $2_2^+$   | $2.17 \times 10^{-6}$         | $1.04 \times 10^{-7}$  | $2.18 \times 10^{-6}$  | $1.05 \times 10^{-7}$  |
|                               |           | $0_2^+$   | $2.19 \times 10^{-8}$         | $5.35 \times 10^{-9}$  | $2.23 \times 10^{-8}$  | $5.38 \times 10^{-9}$  |
|                               | $2_1^+$   | $2_1^+$   |                               |                        | $2.75 \times 10^{-4}$  | $2.64 \times 10^{-6}$  |
|                               |           | $2_2^+$   |                               |                        | $1.24 \times 10^{-7}$  | $4.06 \times 10^{-9}$  |
|                               |           | $2_3^+$   |                               |                        | $8.99 \times 10^{-11}$ | $2.64 \times 10^{-10}$ |
|                               | $3_1^+$   | $2_1^+$   |                               |                        | $1.26 \times 10^{-6}$  | $1.10 \times 10^{-8}$  |
|                               |           | $2_2^+$   |                               |                        | $6.25 \times 10^{-8}$  | $1.74 \times 10^{-9}$  |
|                               |           | $4_1^+$   |                               |                        | $3.04 \times 10^{-6}$  | $3.29 \times 10^{-7}$  |
|                               |           | $4_2^+$   |                               |                        | $1.43 \times 10^{-8}$  | $7.66 \times 10^{-9}$  |
|                               |           | $2_3^+$   |                               |                        | $4.33 \times 10^{-9}$  | $2.66 \times 10^{-9}$  |
|                               | $1_2^+$   | $0_1^+$   |                               |                        | $6.61 \times 10^{-4}$  | $1.97 \times 10^{-6}$  |
|                               |           | $2_1^+$   |                               |                        | $6.91 \times 10^{-4}$  | $5.30 \times 10^{-6}$  |
|                               |           | $2_2^+$   |                               |                        | $1.68 \times 10^{-5}$  | $3.88 \times 10^{-7}$  |
|                               |           | $0_2^+$   |                               |                        | $2.03 \times 10^{-7}$  | $1.28 \times 10^{-8}$  |
|                               |           | $2_3^+$   |                               |                        | $1.55 \times 10^{-8}$  | $4.20 \times 10^{-9}$  |
|                               |           | $2_4^+$   |                               |                        | $4.79 \times 10^{-9}$  | $5.32 \times 10^{-9}$  |
|                               | $2_2^+$   | $2_1^+$   |                               |                        | $1.95 \times 10^{-4}$  | $1.37 \times 10^{-6}$  |
|                               |           | $2_2^+$   |                               |                        | $1.92 \times 10^{-5}$  | $3.90 \times 10^{-7}$  |
|                               |           | $2_3^+$   |                               |                        | $3.36 \times 10^{-8}$  | $6.15 \times 10^{-9}$  |
|                               |           | $2_4^+$   |                               |                        | $1.01 \times 10^{-8}$  | $4.67 \times 10^{-9}$  |

Table (I.A) continued

| Transition Details                          |           |           | $n_e = 1 \times 10^{27} / \text{cm}^3$ |                        |                               |                        |
|---------------------------------------------|-----------|-----------|----------------------------------------|------------------------|-------------------------------|------------------------|
| $Decay$                                     | $J_p^\pi$ | $J_d^\pi$ | $T = 1 \times 10^8 \text{ K}$          |                        | $T = 5 \times 10^8 \text{ K}$ |                        |
|                                             |           |           | $\lambda_c$                            | $\lambda_b$            | $\lambda_c$                   | $\lambda_b$            |
| $^{75}\text{Ge} \rightarrow ^{75}\text{As}$ | $1/2_1^-$ | $3/2_1^-$ | $1.21 \times 10^{-4}$                  | $3.38 \times 10^{-6}$  | $1.22 \times 10^{-4}$         | $3.39 \times 10^{-6}$  |
|                                             |           | $1/2_1^-$ | $6.25 \times 10^{-7}$                  | $2.45 \times 10^{-8}$  | $6.28 \times 10^{-7}$         | $2.46 \times 10^{-8}$  |
|                                             |           | $3/2_2^-$ | $1.57 \times 10^{-5}$                  | $7.00 \times 10^{-7}$  | $1.58 \times 10^{-5}$         | $7.02 \times 10^{-7}$  |
|                                             |           | $1/2_2^-$ | $2.26 \times 10^{-7}$                  | $1.55 \times 10^{-8}$  | $2.27 \times 10^{-7}$         | $1.56 \times 10^{-8}$  |
|                                             |           | $1/2_3^-$ | $4.74 \times 10^{-6}$                  | $4.38 \times 10^{-7}$  | $4.78 \times 10^{-6}$         | $4.39 \times 10^{-7}$  |
|                                             |           | $3/2_3^-$ | $6.63 \times 10^{-7}$                  | $6.71 \times 10^{-8}$  | $6.69 \times 10^{-7}$         | $6.73 \times 10^{-8}$  |
|                                             |           | $3/2_4^-$ | $6.99 \times 10^{-9}$                  | $1.71 \times 10^{-9}$  | $7.12 \times 10^{-9}$         | $1.72 \times 10^{-9}$  |
|                                             |           | $3/2_5^-$ | $8.09 \times 10^{-12}$                 | $8.30 \times 10^{-12}$ | $8.56 \times 10^{-12}$        | $8.44 \times 10^{-12}$ |
|                                             |           | $3/2_6^-$ | $3.49 \times 10^{-10}$                 | $4.18 \times 10^{-10}$ | $3.72 \times 10^{-10}$        | $4.25 \times 10^{-10}$ |
|                                             |           | $1/2_4^-$ | $2.96 \times 10^{-11}$                 | $1.14 \times 10^{-10}$ | $3.39 \times 10^{-11}$        | $1.18 \times 10^{-10}$ |
|                                             |           | $1/2_5^-$ | —                                      | $6.13 \times 10^{-11}$ | —                             | $7.09 \times 10^{-11}$ |
|                                             | $7/2_1^+$ | $9/2_1^+$ |                                        |                        | $3.99 \times 10^{-7}$         | $1.47 \times 10^{-8}$  |
|                                             |           | $5/2_1^+$ |                                        |                        | $5.75 \times 10^{-7}$         | $2.53 \times 10^{-8}$  |
|                                             |           | $5/2_2^+$ |                                        |                        | $6.59 \times 10^{-8}$         | $2.36 \times 10^{-8}$  |
|                                             |           | $5/2_3^+$ |                                        |                        | $6.66 \times 10^{-9}$         | $2.68 \times 10^{-9}$  |
|                                             |           | $9/2_2^+$ |                                        |                        | $1.42 \times 10^{-10}$        | $4.13 \times 10^{-10}$ |
|                                             |           | $5/2_4^+$ |                                        |                        | $1.84 \times 10^{-12}$        | $1.33 \times 10^{-10}$ |
|                                             | $5/2_1^+$ | $5/2_1^+$ |                                        |                        | $2.28 \times 10^{-6}$         | $9.07 \times 10^{-8}$  |
|                                             |           | $5/2_2^+$ |                                        |                        | $1.84 \times 10^{-7}$         | $4.98 \times 10^{-8}$  |
|                                             |           | $5/2_3^+$ |                                        |                        | $8.78 \times 10^{-8}$         | $2.61 \times 10^{-8}$  |
|                                             |           | $5/2_4^+$ |                                        |                        | $1.34 \times 10^{-9}$         | $2.89 \times 10^{-9}$  |
|                                             | $9/2_1^+$ | $9/2_1^+$ |                                        |                        | $1.62 \times 10^{-6}$         | $5.36 \times 10^{-8}$  |
|                                             |           | $9/2_2^+$ |                                        |                        | $6.14 \times 10^{-10}$        | $5.89 \times 10^{-10}$ |
|                                             | $3/2_1^-$ | $3/2_1^-$ |                                        |                        | $7.46 \times 10^{-5}$         | $1.42 \times 10^{-6}$  |
|                                             |           | $1/2_1^-$ |                                        |                        | $3.52 \times 10^{-5}$         | $8.97 \times 10^{-7}$  |
|                                             |           | $3/2_2^-$ |                                        |                        | $9.71 \times 10^{-6}$         | $2.75 \times 10^{-7}$  |
|                                             |           | $5/2_1^-$ |                                        |                        | $1.85 \times 10^{-7}$         | $5.37 \times 10^{-9}$  |
|                                             |           | $1/2_2^-$ |                                        |                        | $1.11 \times 10^{-7}$         | $4.49 \times 10^{-9}$  |
|                                             |           | $5/2_2^-$ |                                        |                        | $6.76 \times 10^{-7}$         | $3.34 \times 10^{-8}$  |
|                                             |           | $1/2_3^-$ |                                        |                        | $2.69 \times 10^{-7}$         | $1.36 \times 10^{-8}$  |
|                                             |           | $3/2_3^-$ |                                        |                        | $1.18 \times 10^{-6}$         | $6.42 \times 10^{-8}$  |
|                                             |           | $3/2_4^-$ |                                        |                        | $3.79 \times 10^{-7}$         | $3.75 \times 10^{-8}$  |
|                                             |           | $3/2_5^-$ |                                        |                        | $2.21 \times 10^{-7}$         | $4.23 \times 10^{-8}$  |
|                                             |           | $3/2_6^-$ |                                        |                        | $1.57 \times 10^{-8}$         | $3.15 \times 10^{-9}$  |
|                                             |           | $1/2_4^-$ |                                        |                        | $2.46 \times 10^{-8}$         | $6.18 \times 10^{-9}$  |
|                                             |           | $1/2_5^-$ |                                        |                        | $1.43 \times 10^{-8}$         | $4.53 \times 10^{-9}$  |
|                                             |           | $3/2_7^-$ |                                        |                        | $1.55 \times 10^{-8}$         | $5.88 \times 10^{-9}$  |
|                                             |           | $3/2_8^-$ |                                        |                        | $2.83 \times 10^{-10}$        | $4.58 \times 10^{-10}$ |
|                                             |           | $3/2_9^-$ |                                        |                        | $5.29 \times 10^{-10}$        | $1.38 \times 10^{-9}$  |
|                                             |           | $5/2_3^-$ |                                        |                        | $2.73 \times 10^{-13}$        | $1.08 \times 10^{-10}$ |

Table (I.A) continued

| Transition Details |           |              | $n_e = 1 \times 10^{27} / \text{cm}^3$ |                        |
|--------------------|-----------|--------------|----------------------------------------|------------------------|
| <i>Decay</i>       | $J_p^\pi$ | $J_d^\pi$    | T = $1 \times 10^8$ K                  |                        |
|                    |           |              | $\lambda_c$                            | $\lambda_b$            |
| $5/2_1^-$          | $3/2_1^-$ | $3/2_1^-$    | $1.39 \times 10^{-5}$                  | $2.44 \times 10^{-7}$  |
|                    |           | $3/2_2^-$    | $6.07 \times 10^{-6}$                  | $1.55 \times 10^{-7}$  |
|                    |           | $5/2_1^-$    | $1.94 \times 10^{-5}$                  | $5.09 \times 10^{-7}$  |
|                    |           | $5/2_2^-$    | $3.53 \times 10^{-6}$                  | $1.54 \times 10^{-7}$  |
|                    |           | $3/2_3^-$    | $5.36 \times 10^{-7}$                  | $2.55 \times 10^{-8}$  |
|                    |           | $7/2_1^-$    | $1.23 \times 10^{-5}$                  | $9.20 \times 10^{-7}$  |
|                    |           | $3/2_4^-$    | $7.04 \times 10^{-8}$                  | $5.87 \times 10^{-9}$  |
|                    |           | $7/2_2^-$    | $4.59 \times 10^{-7}$                  | $6.45 \times 10^{-8}$  |
|                    |           | $3/2_5^-$    | $2.63 \times 10^{-8}$                  | $3.97 \times 10^{-9}$  |
|                    |           | $3/2_6^-$    | $6.01 \times 10^{-11}$                 | $9.42 \times 10^{-12}$ |
|                    |           | $7/2_3^-$    | $1.99 \times 10^{-8}$                  | $3.37 \times 10^{-9}$  |
|                    |           | $7/2_4^-$    | $6.15 \times 10^{-8}$                  | $1.06 \times 10^{-8}$  |
|                    |           | $3/2_7^-$    | $5.44 \times 10^{-9}$                  | $1.45 \times 10^{-9}$  |
|                    |           | $7/2_5^-$    | $1.40 \times 10^{-8}$                  | $7.04 \times 10^{-9}$  |
|                    |           | $3/2_8^-$    | $5.21 \times 10^{-11}$                 | $3.68 \times 10^{-11}$ |
|                    |           | $7/2_6^-$    | $3.82 \times 10^{-10}$                 | $3.37 \times 10^{-10}$ |
|                    |           | $3/2_9^-$    | $1.59 \times 10^{-9}$                  | $2.96 \times 10^{-9}$  |
|                    |           | $3/2_{10}^-$ | $7.64 \times 10^{-11}$                 | $1.80 \times 10^{-10}$ |
| $5/2_2^-$          | $3/2_1^-$ | $3/2_1^-$    | $5.03 \times 10^{-6}$                  | $7.33 \times 10^{-8}$  |
|                    |           | $3/2_2^-$    | $1.06 \times 10^{-7}$                  | $2.20 \times 10^{-9}$  |
|                    |           | $5/2_1^-$    | $3.28 \times 10^{-7}$                  | $6.95 \times 10^{-9}$  |
|                    |           | $5/2_2^-$    | $2.81 \times 10^{-6}$                  | $9.46 \times 10^{-8}$  |
|                    |           | $3/2_3^-$    | $5.12 \times 10^{-8}$                  | $1.87 \times 10^{-9}$  |
|                    |           | $7/2_1^-$    | $4.00 \times 10^{-6}$                  | $2.17 \times 10^{-7}$  |
|                    |           | $3/2_4^-$    | $8.89 \times 10^{-10}$                 | $5.31 \times 10^{-11}$ |
|                    |           | $7/2_2^-$    | $1.10 \times 10^{-7}$                  | $1.02 \times 10^{-8}$  |
|                    |           | $3/2_5^-$    | $4.52 \times 10^{-8}$                  | $4.40 \times 10^{-9}$  |
|                    |           | $3/2_6^-$    | $2.51 \times 10^{-9}$                  | $2.52 \times 10^{-10}$ |
|                    |           | $7/2_3^-$    | $1.89 \times 10^{-7}$                  | $2.02 \times 10^{-8}$  |
|                    |           | $7/2_4^-$    | $1.44 \times 10^{-7}$                  | $1.56 \times 10^{-8}$  |
|                    |           | $3/2_7^-$    | $1.40 \times 10^{-8}$                  | $2.11 \times 10^{-9}$  |
|                    |           | $7/2_5^-$    | $4.16 \times 10^{-10}$                 | $9.49 \times 10^{-11}$ |
|                    |           | $3/2_8^-$    | $1.67 \times 10^{-10}$                 | $4.59 \times 10^{-11}$ |
|                    |           | $7/2_6^-$    | $1.88 \times 10^{-10}$                 | $5.78 \times 10^{-11}$ |
|                    |           | $3/2_9^-$    | $7.32 \times 10^{-9}$                  | $3.00 \times 10^{-9}$  |
|                    |           | $3/2_{10}^-$ | $4.33 \times 10^{-10}$                 | $1.90 \times 10^{-10}$ |
|                    |           | $5/2_3^-$    | $7.00 \times 10^{-13}$                 | $7.68 \times 10^{-12}$ |

Table (I.A) continued

| Transition Details                          |           |              | $n_e = 1 \times 10^{27} / \text{cm}^3$ |                        |                               |                        |
|---------------------------------------------|-----------|--------------|----------------------------------------|------------------------|-------------------------------|------------------------|
| $Decay$                                     | $J_p^\pi$ | $J_d^\pi$    | $T = 1 \times 10^8 \text{ K}$          |                        | $T = 5 \times 10^8 \text{ K}$ |                        |
|                                             |           |              | $\lambda_c$                            | $\lambda_b$            | $\lambda_c$                   | $\lambda_b$            |
| $^{81}\text{Se} \rightarrow ^{81}\text{Br}$ | $1/2_1^-$ | $3/2_1^-$    | $5.77 \times 10^{-4}$                  | $1.03 \times 10^{-5}$  | $5.79 \times 10^{-4}$         | $1.03 \times 10^{-5}$  |
|                                             |           | $1/2_1^-$    | $1.40 \times 10^{-7}$                  | $5.56 \times 10^{-9}$  | $1.41 \times 10^{-7}$         | $5.57 \times 10^{-9}$  |
|                                             |           | $3/2_2^-$    | $5.77 \times 10^{-7}$                  | $2.41 \times 10^{-8}$  | $5.80 \times 10^{-7}$         | $2.41 \times 10^{-8}$  |
|                                             |           | $3/2_3^-$    | $1.04 \times 10^{-6}$                  | $5.05 \times 10^{-8}$  | $1.04 \times 10^{-6}$         | $5.06 \times 10^{-8}$  |
|                                             |           | $3/2_4^-$    | $5.07 \times 10^{-6}$                  | $3.57 \times 10^{-7}$  | $5.11 \times 10^{-6}$         | $3.58 \times 10^{-7}$  |
|                                             |           | $1/2_2^-$    | $1.74 \times 10^{-7}$                  | $2.55 \times 10^{-8}$  | $1.76 \times 10^{-7}$         | $2.56 \times 10^{-8}$  |
|                                             |           | $3/2_5^-$    | $1.80 \times 10^{-8}$                  | $4.85 \times 10^{-9}$  | $1.83 \times 10^{-8}$         | $4.88 \times 10^{-9}$  |
|                                             |           | $3/2_6^-$    | $4.41 \times 10^{-11}$                 | $2.12 \times 10^{-10}$ | $5.09 \times 10^{-11}$        | $2.20 \times 10^{-10}$ |
|                                             |           | $3/2_7^-$    | $7.02 \times 10^{-11}$                 | $4.64 \times 10^{-10}$ | $8.31 \times 10^{-11}$        | $4.84 \times 10^{-10}$ |
|                                             | $7/2_1^+$ | $9/2_1^+$    | $1.56 \times 10^{-7}$                  | $5.20 \times 10^{-9}$  | $1.57 \times 10^{-7}$         | $5.21 \times 10^{-9}$  |
|                                             |           | $7/2_1^+$    | $5.18 \times 10^{-7}$                  | $1.41 \times 10^{-7}$  | $5.28 \times 10^{-7}$         | $1.42 \times 10^{-7}$  |
|                                             |           | $9/2_2^+$    | $1.18 \times 10^{-7}$                  | $9.65 \times 10^{-8}$  | $1.23 \times 10^{-7}$         | $9.78 \times 10^{-8}$  |
|                                             | $9/2_1^+$ | $9/2_1^+$    |                                        |                        | $2.82 \times 10^{-6}$         | $6.97 \times 10^{-8}$  |
|                                             |           | $7/2_1^+$    |                                        |                        | $3.39 \times 10^{-7}$         | $4.52 \times 10^{-8}$  |
|                                             |           | $11/2_1^+$   |                                        |                        | $3.37 \times 10^{-8}$         | $7.64 \times 10^{-9}$  |
|                                             |           | $9/2_2^+$    |                                        |                        | $1.71 \times 10^{-6}$         | $4.20 \times 10^{-7}$  |
|                                             |           | $7/2_2^+$    |                                        |                        | $4.43 \times 10^{-9}$         | $7.08 \times 10^{-9}$  |
|                                             | $3/2_1^-$ | $3/2_1^-$    |                                        |                        | $7.37 \times 10^{-4}$         | $7.65 \times 10^{-6}$  |
|                                             |           | $5/2_1^-$    |                                        |                        | $5.66 \times 10^{-5}$         | $7.98 \times 10^{-7}$  |
|                                             |           | $1/2_1^-$    |                                        |                        | $7.82 \times 10^{-7}$         | $1.53 \times 10^{-8}$  |
|                                             |           | $3/2_2^-$    |                                        |                        | $3.63 \times 10^{-5}$         | $7.36 \times 10^{-7}$  |
|                                             |           | $3/2_3^-$    |                                        |                        | $6.88 \times 10^{-8}$         | $1.56 \times 10^{-9}$  |
|                                             |           | $5/2_2^-$    |                                        |                        | $8.31 \times 10^{-5}$         | $2.24 \times 10^{-6}$  |
|                                             |           | $3/2_4^-$    |                                        |                        | $2.69 \times 10^{-6}$         | $7.95 \times 10^{-8}$  |
|                                             |           | $5/2_3^-$    |                                        |                        | $4.34 \times 10^{-6}$         | $1.77 \times 10^{-7}$  |
|                                             |           | $1/2_2^-$    |                                        |                        | $1.89 \times 10^{-6}$         | $8.97 \times 10^{-8}$  |
|                                             |           | $5/2_4^-$    |                                        |                        | $4.17 \times 10^{-7}$         | $2.33 \times 10^{-8}$  |
|                                             |           | $3/2_5^-$    |                                        |                        | $2.87 \times 10^{-6}$         | $1.88 \times 10^{-7}$  |
|                                             |           | $5/2_5^-$    |                                        |                        | $7.35 \times 10^{-7}$         | $5.48 \times 10^{-8}$  |
|                                             |           | $3/2_6^-$    |                                        |                        | $1.30 \times 10^{-6}$         | $1.57 \times 10^{-7}$  |
|                                             |           | $3/2_7^-$    |                                        |                        | $9.89 \times 10^{-7}$         | $1.28 \times 10^{-7}$  |
|                                             |           | $3/2_8^-$    |                                        |                        | $1.63 \times 10^{-6}$         | $2.17 \times 10^{-7}$  |
|                                             |           | $5/2_6^-$    |                                        |                        | $3.48 \times 10^{-8}$         | $1.28 \times 10^{-8}$  |
|                                             |           | $3/2_9^-$    |                                        |                        | $8.38 \times 10^{-9}$         | $4.76 \times 10^{-9}$  |
|                                             |           | $3/2_{10}^-$ |                                        |                        | $3.66 \times 10^{-8}$         | $2.41 \times 10^{-8}$  |
|                                             | $5/2_1^-$ | $3/2_1^-$    |                                        |                        | $3.33 \times 10^{-7}$         | $3.46 \times 10^{-9}$  |
|                                             |           | $5/2_1^-$    |                                        |                        | $4.61 \times 10^{-4}$         | $6.50 \times 10^{-6}$  |
|                                             |           | $3/2_2^-$    |                                        |                        | $2.81 \times 10^{-6}$         | $5.69 \times 10^{-8}$  |
|                                             |           | $3/2_3^-$    |                                        |                        | $1.21 \times 10^{-6}$         | $2.76 \times 10^{-8}$  |
|                                             |           | $5/2_2^-$    |                                        |                        | $1.83 \times 10^{-5}$         | $4.92 \times 10^{-7}$  |
|                                             |           | $3/2_4^-$    |                                        |                        | $3.55 \times 10^{-7}$         | $1.05 \times 10^{-8}$  |
|                                             |           | $7/2_1^-$    |                                        |                        | $1.65 \times 10^{-5}$         | $4.94 \times 10^{-7}$  |
|                                             |           | $5/2_3^-$    |                                        |                        | $7.17 \times 10^{-7}$         | $2.93 \times 10^{-8}$  |
|                                             |           | $5/2_4^-$    |                                        |                        | $1.09 \times 10^{-6}$         | $6.09 \times 10^{-8}$  |
|                                             |           | $3/2_5^-$    |                                        |                        | $2.01 \times 10^{-8}$         | $1.32 \times 10^{-9}$  |
|                                             |           | $5/2_5^-$    |                                        |                        | $1.81 \times 10^{-6}$         | $1.35 \times 10^{-7}$  |
|                                             |           | $7/2_2^-$    |                                        |                        | $6.31 \times 10^{-6}$         | $7.01 \times 10^{-7}$  |
|                                             |           | $3/2_6^-$    |                                        |                        | $1.40 \times 10^{-7}$         | $1.70 \times 10^{-8}$  |
|                                             |           | $3/2_7^-$    |                                        |                        | $9.89 \times 10^{-9}$         | $1.28 \times 10^{-9}$  |
|                                             |           | $3/2_8^-$    |                                        |                        | $9.60 \times 10^{-8}$         | $1.27 \times 10^{-8}$  |
|                                             |           | $7/2_3^-$    |                                        |                        | $2.26 \times 10^{-7}$         | $4.82 \times 10^{-8}$  |
|                                             |           | $5/2_6^-$    |                                        |                        | $3.14 \times 10^{-9}$         | $1.16 \times 10^{-9}$  |
|                                             |           | $3/2_9^-$    |                                        |                        | $4.45 \times 10^{-10}$        | $2.53 \times 10^{-10}$ |
|                                             |           | $3/2_{10}^-$ |                                        |                        | $1.34 \times 10^{-9}$         | $8.81 \times 10^{-10}$ |
|                                             |           | $7/2_4^-$    |                                        |                        | $1.56 \times 10^{-8}$         | $5.19 \times 10^{-8}$  |
|                                             |           | $3/2_{11}^-$ |                                        |                        | $1.88 \times 10^{-12}$        | $2.39 \times 10^{-11}$ |

TABLE (I.B) Bound state decay rate ( $\lambda_b$  in  $\text{sec}^{-1}$ ) and continuum state decay rate ( $\lambda_c$  in  $\text{sec}^{-1}$ ) variation with free electron density at a temperature  $T = 3 \times 10^8 K$  for each transition. This table does not include the levels that are not populated at this temperature.

| Transition Details                          |           |           |  | $T = 3 \times 10^8 K$                  |                        |                                        |                        |
|---------------------------------------------|-----------|-----------|--|----------------------------------------|------------------------|----------------------------------------|------------------------|
| $Decay$                                     | $J_p^\pi$ | $J_d^\pi$ |  | $n_e = 1 \times 10^{26} / \text{cm}^3$ |                        | $n_e = 1 \times 10^{27} / \text{cm}^3$ |                        |
|                                             |           |           |  | $\lambda_c$                            | $\lambda_b$            | $\lambda_c$                            | $\lambda_b$            |
| $^{65}\text{Ni} \rightarrow ^{65}\text{Cu}$ | $5/2_1^-$ | $3/2_1^-$ |  | $4.52 \times 10^{-5}$                  | $2.81 \times 10^{-7}$  | $4.51 \times 10^{-5}$                  | $2.71 \times 10^{-7}$  |
|                                             |           | $5/2_1^-$ |  | $3.60 \times 10^{-6}$                  | $9.92 \times 10^{-8}$  | $3.59 \times 10^{-6}$                  | $9.58 \times 10^{-8}$  |
|                                             |           | $7/2_1^-$ |  | $2.05 \times 10^{-5}$                  | $1.22 \times 10^{-6}$  | $2.03 \times 10^{-5}$                  | $1.18 \times 10^{-6}$  |
|                                             |           | $5/2_2^-$ |  | $1.81 \times 10^{-6}$                  | $1.59 \times 10^{-7}$  | $1.79 \times 10^{-6}$                  | $1.54 \times 10^{-7}$  |
|                                             |           | $3/2_2^-$ |  | $1.45 \times 10^{-7}$                  | $1.79 \times 10^{-8}$  | $1.43 \times 10^{-7}$                  | $1.72 \times 10^{-8}$  |
|                                             |           | $7/2_2^-$ |  | $2.95 \times 10^{-9}$                  | $8.64 \times 10^{-9}$  | $2.66 \times 10^{-9}$                  | $8.11 \times 10^{-9}$  |
|                                             | $1/2_1^-$ | $5/2_3^-$ |  | $1.65 \times 10^{-12}$                 | $8.93 \times 10^{-12}$ | $1.42 \times 10^{-12}$                 | $8.28 \times 10^{-12}$ |
|                                             |           | $3/2_1^-$ |  | $5.41 \times 10^{-3}$                  | $3.15 \times 10^{-5}$  | $5.40 \times 10^{-3}$                  | $3.05 \times 10^{-5}$  |
|                                             |           | $1/2_1^-$ |  | $2.39 \times 10^{-5}$                  | $3.45 \times 10^{-7}$  | $2.38 \times 10^{-5}$                  | $3.33 \times 10^{-7}$  |
|                                             |           | $3/2_2^-$ |  | $3.16 \times 10^{-7}$                  | $3.13 \times 10^{-8}$  | $3.12 \times 10^{-7}$                  | $3.02 \times 10^{-8}$  |
| $^{66}\text{Cu} \rightarrow ^{66}\text{Zn}$ | $1_1^+$   | $0_1^+$   |  | $1.19 \times 10^{-3}$                  | $5.02 \times 10^{-6}$  | $1.19 \times 10^{-3}$                  | $4.85 \times 10^{-6}$  |
|                                             |           | $2_1^+$   |  | $3.50 \times 10^{-4}$                  | $4.36 \times 10^{-6}$  | $3.49 \times 10^{-4}$                  | $4.21 \times 10^{-6}$  |
|                                             |           | $2_2^+$   |  | $2.19 \times 10^{-6}$                  | $1.08 \times 10^{-7}$  | $2.18 \times 10^{-6}$                  | $1.05 \times 10^{-7}$  |
|                                             |           | $0_2^+$   |  | $2.26 \times 10^{-8}$                  | $5.58 \times 10^{-9}$  | $2.22 \times 10^{-8}$                  | $5.37 \times 10^{-9}$  |
|                                             | $2_1^+$   | $2_1^+$   |  | $2.75 \times 10^{-4}$                  | $2.73 \times 10^{-6}$  | $2.75 \times 10^{-4}$                  | $2.64 \times 10^{-6}$  |
|                                             |           | $2_2^+$   |  | $1.24 \times 10^{-7}$                  | $4.21 \times 10^{-9}$  | $1.24 \times 10^{-7}$                  | $4.06 \times 10^{-9}$  |
|                                             |           | $2_3^+$   |  | $9.63 \times 10^{-11}$                 | $2.78 \times 10^{-10}$ | $8.70 \times 10^{-11}$                 | $2.62 \times 10^{-10}$ |
|                                             | $3_1^+$   | $2_1^+$   |  | $1.27 \times 10^{-6}$                  | $1.13 \times 10^{-8}$  | $1.26 \times 10^{-6}$                  | $1.10 \times 10^{-8}$  |
|                                             |           | $2_2^+$   |  | $6.27 \times 10^{-8}$                  | $1.80 \times 10^{-9}$  | $6.24 \times 10^{-8}$                  | $1.74 \times 10^{-9}$  |
|                                             |           | $4_1^+$   |  | $3.07 \times 10^{-6}$                  | $3.41 \times 10^{-7}$  | $3.03 \times 10^{-6}$                  | $3.29 \times 10^{-7}$  |
|                                             |           | $4_2^+$   |  | $1.47 \times 10^{-8}$                  | $7.97 \times 10^{-9}$  | $1.42 \times 10^{-8}$                  | $7.63 \times 10^{-9}$  |
|                                             |           | $2_3^+$   |  | $4.45 \times 10^{-9}$                  | $2.77 \times 10^{-9}$  | $4.28 \times 10^{-9}$                  | $2.65 \times 10^{-9}$  |

Table (I.B) continued.

| Transition Details            |           |            | $T = 3 \times 10^8 K$           |                        |                                 |                        |
|-------------------------------|-----------|------------|---------------------------------|------------------------|---------------------------------|------------------------|
|                               |           |            | $n_e = 1 \times 10^{26} / cm^3$ |                        | $n_e = 1 \times 10^{27} / cm^3$ |                        |
|                               |           |            | $\lambda_c$                     | $\lambda_b$            | $\lambda_c$                     | $\lambda_b$            |
| $^{75}Ge \rightarrow ^{75}As$ | $1/2_1^-$ | $3/2_1^-$  | $1.22 \times 10^{-4}$           | $3.51 \times 10^{-6}$  | $1.22 \times 10^{-4}$           | $3.38 \times 10^{-6}$  |
|                               |           | $1/2_1^-$  | $6.31 \times 10^{-7}$           | $2.54 \times 10^{-8}$  | $6.27 \times 10^{-7}$           | $2.46 \times 10^{-8}$  |
|                               |           | $3/2_2^-$  | $1.59 \times 10^{-5}$           | $7.27 \times 10^{-7}$  | $1.58 \times 10^{-5}$           | $7.01 \times 10^{-7}$  |
|                               |           | $1/2_2^-$  | $2.29 \times 10^{-7}$           | $1.61 \times 10^{-8}$  | $2.27 \times 10^{-7}$           | $1.56 \times 10^{-8}$  |
|                               |           | $1/2_3^-$  | $4.81 \times 10^{-7}$           | $4.55 \times 10^{-7}$  | $4.77 \times 10^{-6}$           | $4.39 \times 10^{-7}$  |
|                               |           | $3/2_3^-$  | $6.74 \times 10^{-7}$           | $6.97 \times 10^{-8}$  | $6.67 \times 10^{-7}$           | $6.72 \times 10^{-8}$  |
|                               |           | $3/2_4^-$  | $7.21 \times 10^{-9}$           | $1.78 \times 10^{-9}$  | $7.08 \times 10^{-9}$           | $1.72 \times 10^{-9}$  |
|                               |           | $3/2_5^-$  | $8.85 \times 10^{-12}$          | $8.80 \times 10^{-12}$ | $8.43 \times 10^{-12}$          | $8.40 \times 10^{-12}$ |
|                               |           | $3/2_6^-$  | $3.86 \times 10^{-10}$          | $4.44 \times 10^{-10}$ | $3.66 \times 10^{-10}$          | $4.23 \times 10^{-10}$ |
|                               |           | $1/2_4^-$  | $3.63 \times 10^{-11}$          | $1.24 \times 10^{-10}$ | $3.28 \times 10^{-11}$          | $1.17 \times 10^{-10}$ |
|                               |           | $1/2_5^-$  | $5.35 \times 10^{-17}$          | $8.02 \times 10^{-11}$ | —                               | $6.80 \times 10^{-11}$ |
|                               | $7/2_1^+$ | $9/2_1^+$  | $4.01 \times 10^{-7}$           | $1.52 \times 10^{-8}$  | $3.98 \times 10^{-7}$           | $1.47 \times 10^{-8}$  |
|                               |           | $5/2_1^+$  | $5.78 \times 10^{-7}$           | $2.62 \times 10^{-8}$  | $5.75 \times 10^{-7}$           | $2.53 \times 10^{-8}$  |
|                               |           | $5/2_2^+$  | $6.71 \times 10^{-8}$           | $2.45 \times 10^{-8}$  | $6.54 \times 10^{-8}$           | $2.35 \times 10^{-8}$  |
|                               |           | $5/2_3^+$  | $6.78 \times 10^{-9}$           | $2.79 \times 10^{-9}$  | $6.60 \times 10^{-9}$           | $2.68 \times 10^{-9}$  |
|                               |           | $9/2_2^+$  | $1.52 \times 10^{-10}$          | $4.34 \times 10^{-10}$ | $1.38 \times 10^{-10}$          | $4.09 \times 10^{-10}$ |
|                               |           | $5/2_4^+$  | $2.49 \times 10^{-12}$          | $1.44 \times 10^{-10}$ | $1.63 \times 10^{-12}$          | $1.29 \times 10^{-10}$ |
|                               | $5/2_1^+$ | $5/2_1^+$  | $2.29 \times 10^{-6}$           | $9.39 \times 10^{-8}$  | $2.27 \times 10^{-6}$           | $9.07 \times 10^{-8}$  |
|                               |           | $5/2_2^+$  | $1.87 \times 10^{-7}$           | $5.17 \times 10^{-8}$  | $1.83 \times 10^{-7}$           | $4.97 \times 10^{-8}$  |
|                               |           | $5/2_3^+$  | $8.91 \times 10^{-8}$           | $2.71 \times 10^{-8}$  | $8.72 \times 10^{-8}$           | $2.61 \times 10^{-8}$  |
|                               |           | $5/2_4^+$  | $1.41 \times 10^{-9}$           | $3.03 \times 10^{-9}$  | $1.30 \times 10^{-9}$           | $2.86 \times 10^{-9}$  |
|                               | $9/2_1^+$ | $9/2_1^+$  | $1.63 \times 10^{-6}$           | $5.55 \times 10^{-8}$  | $1.62 \times 10^{-6}$           | $5.35 \times 10^{-8}$  |
|                               |           | $9/2_2^+$  | $6.34 \times 10^{-10}$          | $6.14 \times 10^{-10}$ | $6.04 \times 10^{-10}$          | $5.86 \times 10^{-10}$ |
|                               | $3/2_1^-$ | $3/2_1^-$  | $7.48 \times 10^{-5}$           | $1.47 \times 10^{-6}$  | $7.45 \times 10^{-5}$           | $1.42 \times 10^{-6}$  |
|                               |           | $1/2_1^-$  | $3.53 \times 10^{-5}$           | $9.29 \times 10^{-7}$  | $3.51 \times 10^{-5}$           | $8.97 \times 10^{-7}$  |
|                               |           | $3/2_2^-$  | $9.74 \times 10^{-6}$           | $2.85 \times 10^{-7}$  | $9.70 \times 10^{-6}$           | $2.75 \times 10^{-7}$  |
|                               |           | $5/2_1^-$  | $1.86 \times 10^{-7}$           | $5.56 \times 10^{-9}$  | $1.85 \times 10^{-7}$           | $5.37 \times 10^{-9}$  |
|                               |           | $1/2_2^-$  | $1.12 \times 10^{-7}$           | $4.65 \times 10^{-9}$  | $1.11 \times 10^{-7}$           | $4.49 \times 10^{-9}$  |
|                               |           | $5/2_2^-$  | $6.80 \times 10^{-7}$           | $3.46 \times 10^{-8}$  | $6.75 \times 10^{-7}$           | $3.34 \times 10^{-8}$  |
|                               |           | $1/2_3^-$  | $2.71 \times 10^{-7}$           | $1.41 \times 10^{-8}$  | $2.69 \times 10^{-7}$           | $1.36 \times 10^{-8}$  |
|                               |           | $3/2_3^-$  | $1.19 \times 10^{-6}$           | $6.65 \times 10^{-8}$  | $1.18 \times 10^{-6}$           | $6.41 \times 10^{-8}$  |
|                               |           | $3/2_4^-$  | $3.82 \times 10^{-7}$           | $3.89 \times 10^{-8}$  | $3.78 \times 10^{-7}$           | $3.75 \times 10^{-8}$  |
|                               |           | $3/2_5^-$  | $2.24 \times 10^{-7}$           | $4.38 \times 10^{-8}$  | $2.20 \times 10^{-7}$           | $4.22 \times 10^{-8}$  |
|                               |           | $3/2_6^-$  | $1.59 \times 10^{-8}$           | $3.26 \times 10^{-9}$  | $1.57 \times 10^{-8}$           | $3.14 \times 10^{-9}$  |
|                               |           | $1/2_4^-$  | $2.49 \times 10^{-8}$           | $6.42 \times 10^{-8}$  | $2.45 \times 10^{-8}$           | $6.17 \times 10^{-8}$  |
|                               |           | $1/2_5^-$  | $1.46 \times 10^{-8}$           | $4.70 \times 10^{-9}$  | $1.43 \times 10^{-8}$           | $4.52 \times 10^{-9}$  |
|                               |           | $3/2_7^-$  | $1.58 \times 10^{-8}$           | $6.11 \times 10^{-9}$  | $1.54 \times 10^{-8}$           | $5.86 \times 10^{-9}$  |
|                               |           | $3/2_8^-$  | $2.96 \times 10^{-10}$          | $4.79 \times 10^{-10}$ | $2.77 \times 10^{-10}$          | $4.55 \times 10^{-10}$ |
|                               |           | $3/2_9^-$  | $5.61 \times 10^{-10}$          | $1.45 \times 10^{-9}$  | $5.14 \times 10^{-10}$          | $1.37 \times 10^{-9}$  |
|                               |           | $5/2_3^-$  | $4.86 \times 10^{-13}$          | $1.19 \times 10^{-10}$ | $2.16 \times 10^{-13}$          | $1.05 \times 10^{-10}$ |
| $^{81}Se \rightarrow ^{81}Br$ | $1/2_1^-$ | $3/2_1^-$  | $5.80 \times 10^{-4}$           | $1.07 \times 10^{-5}$  | $5.78 \times 10^{-4}$           | $1.03 \times 10^{-5}$  |
|                               |           | $1/2_1^-$  | $1.41 \times 10^{-7}$           | $5.77 \times 10^{-9}$  | $1.40 \times 10^{-7}$           | $5.56 \times 10^{-9}$  |
|                               |           | $3/2_2^-$  | $5.82 \times 10^{-7}$           | $2.50 \times 10^{-8}$  | $5.79 \times 10^{-7}$           | $2.41 \times 10^{-8}$  |
|                               |           | $3/2_3^-$  | $1.05 \times 10^{-6}$           | $5.25 \times 10^{-8}$  | $1.04 \times 10^{-6}$           | $5.06 \times 10^{-8}$  |
|                               |           | $3/2_4^-$  | $5.14 \times 10^{-6}$           | $3.71 \times 10^{-7}$  | $5.10 \times 10^{-6}$           | $3.58 \times 10^{-7}$  |
|                               |           | $1/2_2^-$  | $1.78 \times 10^{-7}$           | $2.66 \times 10^{-8}$  | $1.75 \times 10^{-7}$           | $2.56 \times 10^{-8}$  |
|                               |           | $3/2_5^-$  | $1.85 \times 10^{-8}$           | $5.07 \times 10^{-9}$  | $1.82 \times 10^{-8}$           | $4.88 \times 10^{-9}$  |
|                               |           | $3/2_6^-$  | $5.50 \times 10^{-11}$          | $2.31 \times 10^{-10}$ | $4.92 \times 10^{-11}$          | $2.17 \times 10^{-10}$ |
|                               |           | $3/2_7^-$  | $9.09 \times 10^{-11}$          | $5.11 \times 10^{-10}$ | $7.99 \times 10^{-11}$          | $4.78 \times 10^{-10}$ |
|                               | $7/2_1^+$ | $9/2_1^+$  | $1.58 \times 10^{-7}$           | $5.40 \times 10^{-9}$  | $1.57 \times 10^{-7}$           | $5.21 \times 10^{-9}$  |
|                               |           | $7/2_1^+$  | $5.35 \times 10^{-7}$           | $1.48 \times 10^{-7}$  | $5.25 \times 10^{-7}$           | $1.42 \times 10^{-7}$  |
|                               |           | $9/2_2^+$  | $1.26 \times 10^{-7}$           | $1.02 \times 10^{-7}$  | $1.21 \times 10^{-7}$           | $9.74 \times 10^{-8}$  |
|                               | $9/2_1^+$ | $9/2_1^+$  | $2.83 \times 10^{-6}$           | $7.22 \times 10^{-8}$  | $2.81 \times 10^{-6}$           | $6.97 \times 10^{-8}$  |
|                               |           | $7/2_1^+$  | $3.42 \times 10^{-7}$           | $4.69 \times 10^{-8}$  | $3.38 \times 10^{-7}$           | $4.52 \times 10^{-8}$  |
|                               |           | $11/2_1^+$ | $3.42 \times 10^{-8}$           | $7.92 \times 10^{-9}$  | $3.36 \times 10^{-8}$           | $7.62 \times 10^{-9}$  |
|                               |           | $9/2_2^+$  | $1.73 \times 10^{-6}$           | $4.36 \times 10^{-7}$  | $1.70 \times 10^{-6}$           | $4.19 \times 10^{-7}$  |
|                               |           | $7/2_2^+$  | $4.63 \times 10^{-9}$           | $7.39 \times 10^{-9}$  | $4.35 \times 10^{-9}$           | $7.03 \times 10^{-9}$  |

Table (II) Calculated bare atom  $\beta^-$  decay rate ( $\lambda_k$ , where  $\lambda_k = (\lambda_b + \lambda_c) \times n_{ik}$ ; in  $\text{sec}^{-1}$ ) and branching ( $I_k$ ) from each parent level to daughter level m with branching ( $I_m$ ) for various density - temperature combinations. Here, Column 2: spin-parity of parent energy levels; Column 7 and Column 12: spin-parity of daughter energy levels. Temperature (T) is given in Column 3, Column 8 and Column 13; where  $T_1 = 1 \times 10^8 K$ ,  $T_3 = 3 \times 10^8 K$  and  $T_5 = 5 \times 10^8 K$ , respectively. Column 4: equilibrium population of the k - th nuclear state of the i - th nucleus ( $n_{ik}$ ) at different temperatures. Column 5 and Column 10: Total  $\beta^-$  branching ( $I_k$ ) from each parent level at different density - temperature combinations. Column 6 and Column 11: stellar  $\beta^-$  decay rate ( $\lambda_k$ ) of bare atom i from its k - th nuclear level. Column 9 and Column 14:  $\beta^-$  branching ( $I_m$ ) to each daughter level m.

| Decay                                       | $J_p^\pi$ | T     | $n_{ik}$              | $n_e = 1 \times 10^{26} / \text{cm}^3$ |                       |           |       |           | $n_e = 1 \times 10^{27} / \text{cm}^3$ |                       |           |       |           |
|---------------------------------------------|-----------|-------|-----------------------|----------------------------------------|-----------------------|-----------|-------|-----------|----------------------------------------|-----------------------|-----------|-------|-----------|
|                                             |           |       |                       | $I_k(\%)$                              | $\lambda_k$           | $J_d^\pi$ | T     | $I_m(\%)$ | $I_k(\%)$                              | $\lambda_k$           | $J_d^\pi$ | T     | $I_m(\%)$ |
| $^{65}\text{Ni} \rightarrow ^{65}\text{Cu}$ | $5/2_1^-$ | $T_1$ | $1.00 \times 10^0$    | 98.44                                  | $7.29 \times 10^{-5}$ | $3/2_1^-$ | $T_1$ | 61.29     | 98.43                                  | $7.24 \times 10^{-5}$ | $3/2_1^-$ | $T_1$ | 61.50     |
|                                             |           | $T_3$ | $9.72 \times 10^{-1}$ | 31.79                                  | $7.10 \times 10^{-5}$ |           | $T_3$ | 19.79     | 31.74                                  | $7.06 \times 10^{-5}$ |           | $T_3$ | 19.80     |
|                                             |           | $T_5$ | $9.29 \times 10^{-1}$ | 14.85                                  | $6.69 \times 10^{-5}$ |           | $T_5$ | 9.25      | 14.83                                  | $6.75 \times 10^{-5}$ |           | $T_5$ | 9.25      |
|                                             |           |       |                       |                                        |                       | $5/2_1^-$ | $T_1$ | 4.99      |                                        |                       | $5/2_1^-$ | $T_1$ | 4.99      |
|                                             |           |       |                       |                                        |                       |           | $T_3$ | 1.61      |                                        |                       |           | $T_3$ | 1.61      |
|                                             |           |       |                       |                                        |                       |           | $T_5$ | 0.75      |                                        |                       |           | $T_5$ | 0.75      |
|                                             |           |       |                       |                                        |                       | $7/2_1^-$ | $T_1$ | 29.27     |                                        |                       | $7/2_1^-$ | $T_1$ | 29.09     |
|                                             |           |       |                       |                                        |                       |           | $T_3$ | 9.46      |                                        |                       |           | $T_3$ | 9.40      |
|                                             |           |       |                       |                                        |                       |           | $T_5$ | 4.41      |                                        |                       |           | $T_5$ | 4.40      |
|                                             |           |       |                       |                                        |                       | $5/2_2^-$ | $T_1$ | 2.65      |                                        |                       | $5/2_2^-$ | $T_1$ | 2.62      |
|                                             |           |       |                       |                                        |                       |           | $T_3$ | 0.86      |                                        |                       |           | $T_3$ | 0.85      |
|                                             |           |       |                       |                                        |                       |           | $T_5$ | 0.40      |                                        |                       |           | $T_5$ | 0.40      |
|                                             |           |       |                       |                                        |                       | $3/2_2^-$ | $T_1$ | 0.22      |                                        |                       | $3/2_2^-$ | $T_1$ | 0.22      |
|                                             |           |       |                       |                                        |                       |           | $T_3$ | 0.07      |                                        |                       |           | $T_3$ | 0.07      |
|                                             |           |       |                       |                                        |                       |           | $T_5$ | 0.03      |                                        |                       |           | $T_5$ | 0.03      |
|                                             |           |       |                       |                                        |                       | $7/2_2^-$ | $T_1$ | 0.02      |                                        |                       | $7/2_2^-$ | $T_1$ | 0.01      |
|                                             |           |       |                       |                                        |                       |           | $T_3$ | 0.01      |                                        |                       |           | $T_3$ | 0.00      |
|                                             |           |       |                       |                                        |                       |           | $T_5$ | 0.00      |                                        |                       |           | $T_5$ | 0.00      |
|                                             |           | $T_1$ | $2.12 \times 10^{-4}$ | 1.56                                   | $1.16 \times 10^{-6}$ | $3/2_1^-$ | $T_1$ | 1.56      | 1.57                                   | $1.15 \times 10^{-6}$ | $3/2_1^-$ | $T_1$ | 1.56      |
|                                             |           | $T_3$ | $2.79 \times 10^{-2}$ | 68.21                                  | $1.52 \times 10^{-4}$ |           | $T_3$ | 67.90     | 68.26                                  | $1.52 \times 10^{-4}$ |           | $T_3$ | 67.95     |
|                                             |           | $T_5$ | $7.10 \times 10^{-2}$ | 85.06                                  | $3.83 \times 10^{-4}$ |           | $T_5$ | 84.68     | 85.08                                  | $3.87 \times 10^{-4}$ |           | $T_5$ | 84.69     |
|                                             |           |       |                       |                                        |                       | $1/2_1^-$ | $T_1$ | 0.01      |                                        |                       | $1/2_1^-$ | $T_1$ | 0.01      |
|                                             |           |       |                       |                                        |                       |           | $T_3$ | 0.30      |                                        |                       |           | $T_3$ | 0.30      |
|                                             |           |       |                       |                                        |                       |           | $T_5$ | 0.38      |                                        |                       |           | $T_5$ | 0.38      |
|                                             |           |       |                       |                                        |                       | $3/2_2^-$ | $T_1$ | 0.00      |                                        |                       | $3/2_2^-$ | $T_1$ | 0.00      |
|                                             |           |       |                       |                                        |                       |           | $T_3$ | 0.00      |                                        |                       |           | $T_3$ | 0.00      |
|                                             |           |       |                       |                                        |                       |           | $T_5$ | 0.01      |                                        |                       |           | $T_5$ | 0.01      |
|                                             |           | $T_1$ | $0.00 \times 10^0$    | 0.006                                  | $0.00 \times 10^0$    | $3/2_1^-$ | $T_1$ | 0.00      | 0.00                                   | $0.00 \times 10^0$    | $3/2_1^-$ | $T_1$ | 0.00      |
|                                             |           | $T_3$ | $0.00 \times 10^0$    | 0.00                                   | $0.00 \times 10^0$    |           | $T_3$ | 0.00      | 0.00                                   | $0.00 \times 10^0$    |           | $T_3$ | 0.00      |
|                                             |           | $T_5$ | $4.62 \times 10^{-4}$ | 0.09                                   | $4.11 \times 10^{-7}$ |           | $T_5$ | 0.09      | 0.09                                   | $4.11 \times 10^{-7}$ |           | $T_5$ | 0.09      |

Table (II) continued

|                                             |         |       |                       |        |                       |         |       |       |        |                       |         |       |       |
|---------------------------------------------|---------|-------|-----------------------|--------|-----------------------|---------|-------|-------|--------|-----------------------|---------|-------|-------|
| $^{66}\text{Cu} \rightarrow ^{66}\text{Zn}$ | $1_1^+$ | $T_1$ | $1.00 \times 10^0$    | 100.00 | $1.55 \times 10^{-3}$ | $0_1^+$ | $T_1$ | 77.03 | 100.00 | $1.55 \times 10^{-3}$ | $0_1^+$ | $T_1$ | 77.07 |
|                                             |         | $T_3$ | $9.99 \times 10^{-1}$ | 99.98  | $1.55 \times 10^{-3}$ |         | $T_3$ | 77.01 | 99.98  | $1.55 \times 10^{-3}$ |         | $T_3$ | 77.04 |
|                                             |         | $T_5$ | $9.74 \times 10^{-1}$ | 99.60  | $1.51 \times 10^{-3}$ |         | $T_5$ | 76.72 | 99.59  | $1.51 \times 10^{-3}$ |         | $T_5$ | 76.74 |
|                                             |         |       |                       |        |                       | $2_1^+$ | $T_1$ | 22.82 |        |                       | $2_1^+$ | $T_1$ | 22.78 |
|                                             |         |       |                       |        |                       |         | $T_3$ | 22.81 |        |                       |         | $T_3$ | 22.79 |
|                                             |         |       |                       |        |                       |         | $T_5$ | 22.73 |        |                       |         | $T_5$ | 22.71 |
|                                             |         |       |                       |        |                       | $2_2^+$ | $T_1$ | 0.15  |        |                       | $2_2^+$ | $T_1$ | 0.15  |
|                                             |         |       |                       |        |                       |         | $T_3$ | 0.15  |        |                       |         | $T_3$ | 0.15  |
|                                             |         |       |                       |        |                       |         | $T_5$ | 0.15  |        |                       |         | $T_5$ | 0.15  |
|                                             |         | $T_1$ | $0.00 \times 10^0$    | 0.00   | $0.00 \times 10^0$    | $2_1^+$ | $T_1$ | 0.00  | 0.00   | $0.00 \times 10^0$    | $2_1^+$ | $T_1$ | 0.00  |
|                                             |         | $T_3$ | $1.25 \times 10^{-3}$ | 0.02   | $3.46 \times 10^{-7}$ |         | $T_3$ | 0.02  | 0.02   | $3.45 \times 10^{-7}$ |         | $T_3$ | 0.02  |
|                                             |         | $T_5$ | $2.16 \times 10^{-2}$ | 0.40   | $6.02 \times 10^{-6}$ |         | $T_5$ | 0.40  | 0.40   | $6.00 \times 10^{-6}$ |         | $T_5$ | 0.40  |

Table (II) continued

|                                             |             |                    |                       |                    |                       |             |       |       |                       |                       |             |       |       |       |  |
|---------------------------------------------|-------------|--------------------|-----------------------|--------------------|-----------------------|-------------|-------|-------|-----------------------|-----------------------|-------------|-------|-------|-------|--|
| $^{75}\text{Ge} \rightarrow ^{75}\text{As}$ | $1/2_1^-$   | $T_1$              | $1.00 \times 10^0$    | 100.00             | $1.49 \times 10^{-4}$ | $3/2_1^-$   | $T_1$ | 84.23 | 100.00                | $1.48 \times 10^{-4}$ | $3/2_1^-$   | $T_1$ | 84.29 |       |  |
|                                             |             | $T_3$              | $9.78 \times 10^{-1}$ | 99.97              | $1.46 \times 10^{-4}$ |             | $T_3$ | 84.20 | 99.97                 | $1.45 \times 10^{-4}$ |             | $T_3$ | 84.24 |       |  |
|                                             |             | $T_5$              | $8.03 \times 10^{-1}$ | 99.20              | $1.14 \times 10^{-4}$ |             | $T_5$ | 83.57 | 99.22                 | $1.19 \times 10^{-4}$ |             | $T_5$ | 83.60 |       |  |
| <hr/>                                       |             |                    |                       |                    |                       |             |       |       |                       |                       |             |       |       |       |  |
|                                             | $1/2_1^-$   | $T_1$              | 0.44                  |                    |                       | $1/2_2^-$   | $T_1$ | 0.44  |                       |                       | $1/2_2^-$   | $T_1$ | 0.44  |       |  |
|                                             |             | $T_3$              | 0.44                  |                    |                       |             |       | $T_3$ | 0.44                  |                       |             |       | $T_3$ | 0.44  |  |
|                                             |             | $T_5$              | 0.44                  |                    |                       |             |       | $T_5$ | 0.44                  |                       |             |       | $T_5$ | 0.44  |  |
| <hr/>                                       |             |                    |                       |                    |                       |             |       |       |                       |                       |             |       |       |       |  |
|                                             | $3/2_2^-$   | $T_1$              | 11.14                 |                    |                       | $3/2_2^-$   | $T_1$ | 11.12 |                       |                       | $3/2_2^-$   | $T_1$ | 11.12 |       |  |
|                                             |             | $T_3$              | 11.13                 |                    |                       |             |       | $T_3$ | 11.12                 |                       |             |       | $T_3$ | 11.12 |  |
|                                             |             | $T_5$              | 11.05                 |                    |                       |             |       | $T_5$ | 11.04                 |                       |             |       | $T_5$ | 11.04 |  |
| <hr/>                                       |             |                    |                       |                    |                       |             |       |       |                       |                       |             |       |       |       |  |
|                                             | $1/2_2^-$   | $T_1$              | 0.16                  |                    |                       | $1/2_2^-$   | $T_1$ | 0.16  |                       |                       | $1/2_2^-$   | $T_1$ | 0.16  |       |  |
|                                             |             | $T_3$              | 0.16                  |                    |                       |             |       | $T_3$ | 0.16                  |                       |             |       | $T_3$ | 0.16  |  |
|                                             |             | $T_5$              | 16.00                 |                    |                       |             |       | $T_5$ | 0.16                  |                       |             |       | $T_5$ | 0.16  |  |
| <hr/>                                       |             |                    |                       |                    |                       |             |       |       |                       |                       |             |       |       |       |  |
|                                             | $1/2_3^-$   | $T_1$              | 3.53                  |                    |                       | $1/2_3^-$   | $T_1$ | 3.53  |                       |                       | $1/2_3^-$   | $T_1$ | 3.50  |       |  |
|                                             |             | $T_3$              | 3.53                  |                    |                       |             |       | $T_3$ | 3.51                  |                       |             |       | $T_3$ | 3.51  |  |
|                                             |             | $T_5$              | 3.50                  |                    |                       |             |       | $T_5$ | 3.48                  |                       |             |       | $T_5$ | 3.48  |  |
| <hr/>                                       |             |                    |                       |                    |                       |             |       |       |                       |                       |             |       |       |       |  |
|                                             | $3/2_3^-$   | $T_1$              | 0.50                  |                    |                       | $3/2_3^-$   | $T_1$ | 0.49  |                       |                       | $3/2_3^-$   | $T_1$ | 0.49  |       |  |
|                                             |             | $T_3$              | 0.50                  |                    |                       |             |       | $T_3$ | 0.49                  |                       |             |       | $T_3$ | 0.49  |  |
|                                             |             | $T_5$              | 0.49                  |                    |                       |             |       | $T_5$ | 0.49                  |                       |             |       | $T_5$ | 0.49  |  |
| <hr/>                                       |             |                    |                       |                    |                       |             |       |       |                       |                       |             |       |       |       |  |
|                                             | $3/2_4^-$   | $T_1$              | 0.01                  |                    |                       | $3/2_4^-$   | $T_1$ | 0.01  |                       |                       | $3/2_4^-$   | $T_1$ | 0.01  |       |  |
|                                             |             | $T_3$              | 0.01                  |                    |                       |             |       | $T_3$ | 0.01                  |                       |             |       | $T_3$ | 0.01  |  |
|                                             |             | $T_5$              | 0.01                  |                    |                       |             |       | $T_5$ | 0.01                  |                       |             |       | $T_5$ | 0.01  |  |
| <hr/>                                       |             |                    |                       |                    |                       |             |       |       |                       |                       |             |       |       |       |  |
| $7/2_1^+$                                   | $T_1$       | $0.00 \times 10^0$ | 0.00                  | $0.00 \times 10^0$ | $5/2_1^+$             | $T_1$       | 0.00  | 0.00  | $0.00 \times 10^0$    | $5/2_1^+$             | $T_1$       | 0.00  |       |       |  |
|                                             |             | $T_3$              | $1.76 \times 10^{-2}$ | 0.02               | $1.97 \times 10^{-8}$ | $T_3$       | 0.01  | 0.01  | $1.96 \times 10^{-8}$ | $T_3$                 | 0.01        |       |       |       |  |
|                                             |             | $T_5$              | $1.25 \times 10^{-1}$ | 0.12               | $1.41 \times 10^{-7}$ | $T_5$       | 0.04  | 0.12  | $1.40 \times 10^{-7}$ | $T_5$                 | 0.04        |       |       |       |  |
| <hr/>                                       |             |                    |                       |                    |                       |             |       |       |                       |                       |             |       |       |       |  |
|                                             | $(5/2_2^+)$ | $T_1$              | 0.00                  |                    |                       | $(5/2_2^+)$ | $T_1$ | 0.00  |                       |                       | $(5/2_2^+)$ | $T_1$ | 0.00  |       |  |
|                                             |             | $T_3$              | 0.01                  |                    |                       |             |       | $T_3$ | 0.01                  |                       |             |       | $T_3$ | 0.01  |  |
|                                             |             | $T_5$              | 0.06                  |                    |                       |             |       | $T_5$ | 0.06                  |                       |             |       | $T_5$ | 0.06  |  |
| <hr/>                                       |             |                    |                       |                    |                       |             |       |       |                       |                       |             |       |       |       |  |
| $5/2_1^+$                                   | $T_1$       | $0.00 \times 10^0$ | 0.00                  | $0.00 \times 10^0$ | $5/2_1^+$             | $T_1$       | 0.00  | 0.00  | $0.00 \times 10^0$    | $5/2_1^+$             | $T_1$       | 0.00  |       |       |  |
|                                             |             | $T_3$              | $0.00 \times 10^0$    | 0.00               | $0.00 \times 10^0$    | $T_3$       | 0.00  | 0.00  | $0.00 \times 10^0$    | $T_3$                 | 0.00        |       |       |       |  |
|                                             |             | $T_5$              | $2.78 \times -2$      | 0.06               | $7.62 \times 10^{-8}$ | $T_5$       | 0.05  | 0.06  | $7.56 \times 10^{-8}$ | $T_5$                 | 0.05        |       |       |       |  |
| <hr/>                                       |             |                    |                       |                    |                       |             |       |       |                       |                       |             |       |       |       |  |
|                                             | $(5/2_2^+)$ | $T_1$              | 0.00                  |                    |                       | $(5/2_2^+)$ | $T_1$ | 0.00  |                       |                       | $(5/2_2^+)$ | $T_1$ | 0.00  |       |  |
|                                             |             | $T_3$              | 0.00                  |                    |                       |             |       | $T_3$ | 0.00                  |                       |             |       | $T_3$ | 0.00  |  |
|                                             |             | $T_5$              | 0.01                  |                    |                       |             |       | $T_5$ | 0.01                  |                       |             |       | $T_5$ | 0.01  |  |
| <hr/>                                       |             |                    |                       |                    |                       |             |       |       |                       |                       |             |       |       |       |  |
| $9/2_1^+$                                   | $T_1$       | $0.00 \times 10^0$ | 0.00                  | $0.00 \times 10^0$ | $9/2_1^+$             | $T_1$       | 0.00  | 0.00  | $0.00 \times 10^0$    | $9/2_1^+$             | $T_1$       | 0.00  |       |       |  |
|                                             |             | $T_3$              | $2.14 \times 10^{-3}$ | 0.00               | $0.00 \times 10^0$    | $T_3$       | 0.00  | 0.00  | $0.00 \times 10^0$    | $T_3$                 | 0.00        |       |       |       |  |
|                                             |             | $T_5$              | $3.88 \times 10^{-2}$ | 0.06               | $6.53 \times 10^{-8}$ | $T_5$       | 0.06  | 0.05  | $6.49 \times 10^{-8}$ | $T_5$                 | 0.05        |       |       |       |  |
| <hr/>                                       |             |                    |                       |                    |                       |             |       |       |                       |                       |             |       |       |       |  |
| $3/2_1^-$                                   | $T_1$       | $0.00 \times 10^0$ | 0.00                  | $0.00 \times 10^0$ | $3/2_1^-$             | $T_1$       | 0.00  | 0.00  | $0.00 \times 10^0$    | $3/2_1^-$             | $T_1$       | 0.00  |       |       |  |
|                                             |             | $T_3$              | $1.09 \times 10^{-4}$ | 0.01               | $1.37 \times 10^{-8}$ | $T_3$       | 0.01  | 0.01  | $1.36 \times 10^{-8}$ | $T_3$                 | 0.01        |       |       |       |  |
|                                             |             | $T_5$              | $4.50 \times 10^{-3}$ | 0.47               | $5.67 \times 10^{-7}$ | $T_5$       | 0.28  | 0.47  | $5.64 \times 10^{-7}$ | $T_5$                 | 0.28        |       |       |       |  |
| <hr/>                                       |             |                    |                       |                    |                       |             |       |       |                       |                       |             |       |       |       |  |
|                                             | $1/2_1^-$   | $T_1$              | 0.00                  |                    |                       | $1/2_1^-$   | $T_1$ | 0.00  |                       |                       | $1/2_1^-$   | $T_1$ | 0.00  |       |  |
|                                             |             | $T_3$              | 0.00                  |                    |                       |             |       | $T_3$ | 0.00                  |                       |             |       | $T_3$ | 0.00  |  |
|                                             |             | $T_5$              | 0.13                  |                    |                       |             |       | $T_5$ | 0.13                  |                       |             |       | $T_5$ | 0.13  |  |
| <hr/>                                       |             |                    |                       |                    |                       |             |       |       |                       |                       |             |       |       |       |  |
|                                             | $3/2_2^-$   | $T_1$              | 0.00                  |                    |                       | $3/2_2^-$   | $T_1$ | 0.00  |                       |                       | $3/2_2^-$   | $T_1$ | 0.00  |       |  |
|                                             |             | $T_3$              | 0.00                  |                    |                       |             |       | $T_3$ | 0.00                  |                       |             |       | $T_3$ | 0.00  |  |
|                                             |             | $T_5$              | 0.04                  |                    |                       |             |       | $T_5$ | 0.04                  |                       |             |       | $T_5$ | 0.04  |  |
| <hr/>                                       |             |                    |                       |                    |                       |             |       |       |                       |                       |             |       |       |       |  |
| $5/2_1^-$                                   | $T_1$       | $0.00 \times 10^0$ | 0.00                  | $0.00 \times 10^0$ | $3/2_1^-$             | $T_1$       | 0.00  | 0.00  | $0.00 \times 10^0$    | $3/2_1^-$             | $T_1$       | 0.00  |       |       |  |
|                                             |             | $T_3$              | $1.39 \times 10^{-5}$ | 0.00               | $0.00 \times 10^0$    | $T_3$       | 0.00  | 0.00  | $0.00 \times 10^0$    | $T_3$                 | 0.00        |       |       |       |  |
|                                             |             | $T_5$              | $1.54 \times 10^{-3}$ | 0.07               | $9.05 \times 10^{-8}$ | $T_5$       | 0.02  | 0.07  | $9.00 \times 10^{-8}$ | $T_5$                 | 0.02        |       |       |       |  |
| <hr/>                                       |             |                    |                       |                    |                       |             |       |       |                       |                       |             |       |       |       |  |
|                                             | $3/2_2^-$   | $T_1$              | 0.00                  |                    |                       | $3/2_2^-$   | $T_1$ | 0.00  |                       |                       | $3/2_2^-$   | $T_1$ | 0.00  |       |  |
|                                             |             | $T_3$              | 0.00                  |                    |                       |             |       | $T_3$ | 0.00                  |                       |             |       | $T_3$ | 0.00  |  |
|                                             |             | $T_5$              | 0.01                  |                    |                       |             |       | $T_5$ | 0.01                  |                       |             |       | $T_5$ | 0.01  |  |
| <hr/>                                       |             |                    |                       |                    |                       |             |       |       |                       |                       |             |       |       |       |  |
|                                             | $5/2_1^-$   | $T_1$              | 0.00                  |                    |                       | $5/2_1^-$   | $T_1$ | 0.00  |                       |                       | $5/2_1^-$   | $T_1$ | 0.00  |       |  |
|                                             |             | $T_3$              | 0.00                  |                    |                       |             |       | $T_3$ | 0.00                  |                       |             |       | $T_3$ | 0.00  |  |
|                                             |             | $T_5$              | 0.03                  |                    |                       |             |       | $T_5$ | 0.02                  |                       |             |       | $T_5$ | 0.02  |  |
| <hr/>                                       |             |                    |                       |                    |                       |             |       |       |                       |                       |             |       |       |       |  |
|                                             | $7/2_1^-$   | $T_1$              | 0.00                  |                    |                       | $7/2_1^-$   | $T_1$ | 0.00  |                       |                       | $7/2_1^-$   | $T_1$ | 0.00  |       |  |
|                                             |             | $T_3$              | 0.00                  |                    |                       |             |       | $T_3$ | 0.00                  |                       |             |       | $T_3$ | 0.00  |  |
|                                             |             | $T_5$              | 0.02                  |                    |                       |             |       | $T_5$ | 0.02                  |                       |             |       | $T_5$ | 0.02  |  |

Table (II) continued

|                                             |             |       |                       |        |                       |             |       |       |        |                       |             |       |       |
|---------------------------------------------|-------------|-------|-----------------------|--------|-----------------------|-------------|-------|-------|--------|-----------------------|-------------|-------|-------|
| $^{81}\text{Se} \rightarrow ^{81}\text{Br}$ | $1/2_1^-$   | $T_1$ | $1.00 \times 10^0$    | 100.00 | $5.86 \times 10^{-4}$ | $3/2_1^-$   | $T_1$ | 98.74 | 100.00 | $5.95 \times 10^{-4}$ | $3/2_1^-$   | $T_1$ | 98.74 |
|                                             |             | $T_3$ | $9.31 \times 10^{-1}$ | 99.99  | $5.46 \times 10^{-4}$ |             | $T_3$ | 98.72 | 99.99  | $5.55 \times 10^{-4}$ |             | $T_3$ | 98.73 |
|                                             |             | $T_5$ | $7.29 \times 10^{-1}$ | 99.90  | $4.28 \times 10^{-4}$ |             | $T_5$ | 98.65 | 99.92  | $4.35 \times 10^{-4}$ |             | $T_5$ | 98.66 |
|                                             |             |       |                       |        |                       | $1/2_1^-$   | $T_1$ | 0.02  |        |                       | $1/2_1^-$   | $T_1$ | 0.02  |
|                                             |             |       |                       |        |                       |             | $T_3$ | 0.02  |        |                       |             | $T_3$ | 0.02  |
|                                             |             |       |                       |        |                       |             | $T_5$ | 0.02  |        |                       |             | $T_5$ | 0.02  |
|                                             |             |       |                       |        |                       | $3/2_2^-$   | $T_1$ | 0.10  |        |                       | $3/2_2^-$   | $T_1$ | 0.10  |
|                                             |             |       |                       |        |                       |             | $T_3$ | 0.10  |        |                       |             | $T_3$ | 0.10  |
|                                             |             |       |                       |        |                       |             | $T_5$ | 0.10  |        |                       |             | $T_5$ | 0.10  |
|                                             | $(3/2^-)_3$ | $T_1$ |                       |        |                       | $(3/2^-)_3$ | $T_1$ | 0.18  |        |                       | $(3/2^-)_3$ | $T_1$ | 0.18  |
|                                             |             | $T_3$ |                       |        |                       |             | $T_3$ | 0.18  |        |                       |             | $T_3$ | 0.18  |
|                                             |             | $T_5$ |                       |        |                       |             | $T_5$ | 0.18  |        |                       |             | $T_5$ | 0.18  |
|                                             |             |       |                       |        |                       | $3/2_4^-$   | $T_1$ | 0.92  |        |                       | $3/2_4^-$   | $T_1$ | 0.91  |
|                                             |             |       |                       |        |                       |             | $T_3$ | 0.92  |        |                       |             | $T_3$ | 0.92  |
|                                             |             |       |                       |        |                       |             | $T_5$ | 0.92  |        |                       |             | $T_5$ | 0.92  |
|                                             |             |       |                       |        |                       | $1/2_2^-$   | $T_1$ | 0.03  |        |                       | $1/2_2^-$   | $T_1$ | 0.03  |
|                                             |             |       |                       |        |                       |             | $T_3$ | 0.03  |        |                       |             | $T_3$ | 0.03  |
|                                             |             |       |                       |        |                       |             | $T_5$ | 0.03  |        |                       |             | $T_5$ | 0.03  |
|                                             | $7/2_1^+$   | $T_1$ | $2.56 \times 10^{-5}$ | 0.00   | $0.00 \times 10^0$    | $9/2_1^+$   | $T_1$ | 0.00  | 0.00   | $0.00 \times 10^0$    | $9/2_1^+$   | $T_1$ | 0.00  |
|                                             |             | $T_3$ | $6.92 \times 10^{-2}$ | 0.01   | $7.30 \times 10^{-8}$ |             | $T_3$ | 0.00  | 0.01   | $7.17 \times 10^{-8}$ |             | $T_3$ | 0.00  |
|                                             |             | $T_5$ | $2.67 \times 10^{-1}$ | 0.07   | $2.82 \times 10^{-7}$ |             | $T_5$ | 0.01  | 0.07   | $2.81 \times 10^{-7}$ |             | $T_5$ | 0.01  |
|                                             |             |       |                       |        |                       | $7/2_1^+$   | $T_1$ | 0.00  |        |                       | $7/2_1^+$   | $T_1$ | 0.00  |
|                                             |             |       |                       |        |                       |             | $T_3$ | 0.01  |        |                       |             | $T_3$ | 0.01  |
|                                             |             |       |                       |        |                       |             | $T_5$ | 0.04  |        |                       |             | $T_5$ | 0.04  |
|                                             |             |       |                       |        |                       | $9/2_2^+$   | $T_1$ | 0.00  |        |                       | $9/2_2^+$   | $T_1$ | 0.00  |
|                                             |             |       |                       |        |                       |             | $T_3$ | 0.00  |        |                       |             | $T_3$ | 0.00  |
|                                             |             |       |                       |        |                       |             | $T_5$ | 0.01  |        |                       |             | $T_5$ | 0.01  |

TABLE (III.A) Variation of bound state  $\beta^-$  decay contribution (in %) for individual transitions and to the total decay with temperature at a free electron density. Column 5 and Column 7: Bound state  $\beta^-$  decay contribution in individual transition. Column 6 and Column 8: contribution to total decay rate from bound state decay. See text for more details.

| Transition Details                          |           |           |             | $n = 1 \times 10^{27} / \text{cm}^3$                                       |                                                                         |                                                                            |                                                                         |
|---------------------------------------------|-----------|-----------|-------------|----------------------------------------------------------------------------|-------------------------------------------------------------------------|----------------------------------------------------------------------------|-------------------------------------------------------------------------|
|                                             |           |           |             | T = $1 \times 10^8$ K                                                      |                                                                         | T = $5 \times 10^8$                                                        |                                                                         |
| Decay                                       | $J_p^\pi$ | $J_d^\pi$ | $Q_n$ (keV) | Bound State<br>Decay<br>Contribution<br>(%) in<br>Individual<br>Transition | Bound State<br>Decay<br>Contribution<br>(%) in Total<br>$\beta^-$ Decay | Bound State<br>Decay<br>Contribution<br>(%) in<br>Individual<br>Transition | Bound State<br>Decay<br>Contribution<br>(%) in Total<br>$\beta^-$ Decay |
| $^{65}\text{Ni} \rightarrow ^{65}\text{Cu}$ | $5/2_1^-$ | $3/2_1^-$ | 2137.9      | 0.60                                                                       | 2.35                                                                    | 0.60                                                                       | 0.83                                                                    |
|                                             |           | $5/2_1^-$ | 1022.3      | 2.61                                                                       |                                                                         | 2.60                                                                       |                                                                         |
|                                             |           | $7/2_1^-$ | 656.1       | 5.50                                                                       |                                                                         | 5.47                                                                       |                                                                         |
|                                             |           | $5/2_2^-$ | 514.5       | 7.93                                                                       |                                                                         | 7.89                                                                       |                                                                         |
|                                             |           | $3/2_2^-$ | 2132.9      | 10.78                                                                      |                                                                         | 10.70                                                                      |                                                                         |
|                                             |           | $7/2_2^-$ | 43.56       | 76.84                                                                      |                                                                         | 74.86                                                                      |                                                                         |
|                                             |           | $5/2_3^-$ | 30.5        | 86.82                                                                      |                                                                         | 84.95                                                                      |                                                                         |
|                                             |           | $1/2_1^-$ | 2201.27     | 0.56                                                                       |                                                                         | 0.56                                                                       |                                                                         |
|                                             | $1/2_1^-$ | $1/2_1^-$ | 1430.63     | 1.38                                                                       |                                                                         | 1.38                                                                       |                                                                         |
|                                             |           | $3/2_2^-$ | 476.27      | 8.86                                                                       |                                                                         | 8.80                                                                       |                                                                         |
|                                             |           | $1/2_2^-$ | -11.53      | 100.00                                                                     |                                                                         | 100.00                                                                     |                                                                         |
|                                             |           | $3/2_1^-$ | 2447.98     |                                                                            |                                                                         | 0.44                                                                       |                                                                         |
|                                             | $3/2_1^-$ | $1/2_1^-$ | 1677.34     |                                                                            |                                                                         | 1.00                                                                       |                                                                         |
|                                             |           | $5/2_1^-$ | 1332.48     |                                                                            |                                                                         | 1.59                                                                       |                                                                         |
|                                             |           | $5/2_2^-$ | 824.58      |                                                                            |                                                                         | 3.78                                                                       |                                                                         |
|                                             |           | $3/2_2^-$ | 722.98      |                                                                            |                                                                         | 4.69                                                                       |                                                                         |
|                                             |           | $5/2_3^-$ | 340.58      |                                                                            |                                                                         | 13.73                                                                      |                                                                         |
|                                             |           | $1/2_2^-$ | 235.18      |                                                                            |                                                                         | 21.17                                                                      |                                                                         |
|                                             |           | $3/2_3^-$ | 118.93      |                                                                            |                                                                         | 40.46                                                                      |                                                                         |
|                                             |           | $0_1^+$   | 2640.9      | 0.41                                                                       | 0.59                                                                    | 0.41                                                                       | 0.59                                                                    |
| $^{66}\text{Cu} \rightarrow ^{66}\text{Zn}$ | $1_1^+$   | $2_1^+$   | 1601.7      | 1.20                                                                       |                                                                         | 1.19                                                                       |                                                                         |
|                                             |           | $2_2^+$   | 768.1       | 4.60                                                                       |                                                                         | 4.58                                                                       |                                                                         |
|                                             |           | $0_2^+$   | 269.5       | 19.65                                                                      |                                                                         | 19.43                                                                      |                                                                         |
|                                             |           | $2_1^+$   | 1787.65     |                                                                            |                                                                         | 0.95                                                                       |                                                                         |
|                                             | $2_1^+$   | $2_2^+$   | 954.088     |                                                                            |                                                                         | 3.18                                                                       | 74.62                                                                   |
|                                             |           | $2_3^+$   | 46.696      |                                                                            |                                                                         |                                                                            |                                                                         |
|                                             |           | $2_1^+$   | 1876.7      |                                                                            |                                                                         | 0.86                                                                       |                                                                         |
|                                             | $3_1^+$   | $2_2^+$   | 1043.7      |                                                                            |                                                                         | 2.71                                                                       | 34.84                                                                   |
|                                             |           | $4_1^+$   | 464.9       |                                                                            |                                                                         | 9.76                                                                       |                                                                         |
|                                             |           | $4_2^+$   | 150.34      |                                                                            |                                                                         | 34.84                                                                      |                                                                         |
|                                             |           | $2_3^+$   | 135.743     |                                                                            |                                                                         | 38.06                                                                      |                                                                         |
|                                             |           | $0_1^+$   | 3026.68     |                                                                            |                                                                         | 0.30                                                                       | 52.61                                                                   |
|                                             | $1_2^+$   | $2_1^+$   | 1987.48     |                                                                            |                                                                         | 0.76                                                                       |                                                                         |
|                                             |           | $2_2^+$   | 1154.48     |                                                                            |                                                                         | 2.25                                                                       |                                                                         |
|                                             |           | $0_2^+$   | 654.982     |                                                                            |                                                                         | 5.92                                                                       |                                                                         |
|                                             |           | $2_3^+$   | 246.525     |                                                                            |                                                                         | 21.37                                                                      |                                                                         |
|                                             |           | $2_4^+$   | 88.608      |                                                                            |                                                                         | 52.61                                                                      |                                                                         |
|                                             | $2_2^+$   | $2_1^+$   | 2066.87     |                                                                            |                                                                         | 0.70                                                                       | 15.48                                                                   |
|                                             |           | $2_2^+$   | 1233.87     |                                                                            |                                                                         | 1.99                                                                       |                                                                         |
|                                             |           | $2_3^+$   | 325.905     |                                                                            |                                                                         | 15.48                                                                      |                                                                         |
|                                             |           | $2_4^+$   | 167.995     |                                                                            |                                                                         | 31.50                                                                      |                                                                         |

Table (III.A) continued.

| Transition Details                          |           |           |                   | $n = 1 \times 10^{27} / \text{cm}^3$            |                                                 |                                                 |                                                 |
|---------------------------------------------|-----------|-----------|-------------------|-------------------------------------------------|-------------------------------------------------|-------------------------------------------------|-------------------------------------------------|
|                                             |           |           |                   | T = $1 \times 10^8$ K                           |                                                 | T = $5 \times 10^8$                             |                                                 |
| Decay                                       | $J_p^\pi$ | $J_d^\pi$ | $Q_n(\text{keV})$ | Bound State                                     | Bound State                                     | Bound State                                     | Bound State                                     |
|                                             |           |           |                   | Decay Contribution (%) in Individual Transition | Decay Contribution (%) in Total $\beta^-$ Decay | Decay Contribution (%) in Individual Transition | Decay Contribution (%) in Total $\beta^-$ Decay |
| $^{75}\text{Ge} \rightarrow ^{75}\text{As}$ | $1/2_1^-$ | $3/2_1^-$ | 1177.2            | 2.71                                            | 3.13                                            | 2.70                                            | 3.12                                            |
|                                             |           | $1/2_1^-$ | 978.594           | 3.78                                            |                                                 | 3.76                                            |                                                 |
|                                             |           | $3/2_2^-$ | 912.542           | 4.26                                            |                                                 | 4.25                                            |                                                 |
|                                             |           | $1/2_2^-$ | 708.46            | 6.44                                            |                                                 | 6.41                                            |                                                 |
|                                             |           | $1/2_3^-$ | 592.2             | 8.46                                            |                                                 | 8.42                                            |                                                 |
|                                             |           | $3/2_3^-$ | 559.52            | 9.19                                            |                                                 | 9.14                                            |                                                 |
|                                             |           | $3/2_4^-$ | 311.8             | 19.66                                           |                                                 | 19.47                                           |                                                 |
|                                             |           | $3/2_5^-$ | 113.9             | 50.66                                           |                                                 | 49.64                                           |                                                 |
|                                             |           | $3/2_6^-$ | 102.7             | 54.47                                           |                                                 | 53.33                                           |                                                 |
|                                             |           | $1/2_4^-$ | 50.2              | 79.38                                           |                                                 | 77.67                                           |                                                 |
|                                             |           | $1/2_5^-$ | 5.2               | 100.00                                          |                                                 | 100.00                                          |                                                 |
|                                             | $7/2_1^+$ | $9/2_1^+$ | 1012.97           |                                                 |                                                 | 3.54                                            |                                                 |
|                                             |           | $5/2_1^+$ | 916.232           |                                                 |                                                 | 4.22                                            |                                                 |
|                                             |           | $5/2_2^+$ | 236.09            |                                                 |                                                 | 26.36                                           |                                                 |
|                                             |           | $5/2_3^+$ | 216.69            |                                                 |                                                 | 28.74                                           |                                                 |
|                                             |           | $9/2_2^+$ | 55.88             |                                                 |                                                 | 74.37                                           |                                                 |
|                                             |           | $5/2_4^+$ | 14.59             |                                                 |                                                 | 98.63                                           |                                                 |
|                                             | $5/2_1^+$ | $5/2_1^+$ | 968.732           |                                                 |                                                 | 3.83                                            |                                                 |
|                                             |           | $5/2_2^+$ | 288.59            |                                                 |                                                 | 21.26                                           |                                                 |
|                                             |           | $5/2_3^+$ | 269.19            |                                                 |                                                 | 22.95                                           |                                                 |
|                                             |           | $5/2_4^+$ | 67.09             |                                                 |                                                 | 68.35                                           |                                                 |
|                                             | $9/2_1^+$ | $9/2_1^+$ | 1073.17           |                                                 |                                                 | 3.20                                            |                                                 |
|                                             |           | $9/2_2^+$ | 116.09            |                                                 |                                                 | 48.97                                           |                                                 |
|                                             | $3/2_1^-$ | $3/2_1^-$ | 1430.35           |                                                 |                                                 | 1.87                                            |                                                 |
|                                             |           | $1/2_1^-$ | 1231.74           |                                                 |                                                 | 2.49                                            |                                                 |
|                                             |           | $3/2_2^-$ | 1165.69           |                                                 |                                                 | 2.75                                            |                                                 |
|                                             |           | $5/2_1^-$ | 1150.81           |                                                 |                                                 | 2.82                                            |                                                 |
|                                             |           | $1/2_2^-$ | 961.61            |                                                 |                                                 | 3.88                                            |                                                 |
|                                             |           | $5/2_2^-$ | 857.94            |                                                 |                                                 | 4.71                                            |                                                 |
|                                             |           | $1/2_3^-$ | 845.35            |                                                 |                                                 | 4.83                                            |                                                 |
|                                             |           | $3/2_3^-$ | 812.67            |                                                 |                                                 | 5.15                                            |                                                 |
|                                             |           | $3/2_4^-$ | 564.95            |                                                 |                                                 | 9.01                                            |                                                 |
|                                             |           | $3/2_5^-$ | 367.05            |                                                 |                                                 | 16.03                                           |                                                 |
|                                             |           | $3/2_6^-$ | 355.85            |                                                 |                                                 | 16.65                                           |                                                 |
|                                             |           | $1/2_4^-$ | 303.35            |                                                 |                                                 | 20.09                                           |                                                 |
|                                             |           | $1/2_5^-$ | 258.35            |                                                 |                                                 | 23.99                                           |                                                 |
|                                             |           | $3/2_7^-$ | 226.85            |                                                 |                                                 | 27.45                                           |                                                 |
|                                             |           | $3/2_8^-$ | 80.95             |                                                 |                                                 | 61.83                                           |                                                 |
|                                             |           | $3/2_9^-$ | 59.55             |                                                 |                                                 | 73.32                                           |                                                 |
|                                             |           | $5/2_3^-$ | 10.15             |                                                 |                                                 | 99.75                                           |                                                 |

Table (III.A) continued.

| Transition Details                          |           |              |                   | $1 \times 10^{27} / \text{cc}$                  |                                                 |                                                 |                                                 |
|---------------------------------------------|-----------|--------------|-------------------|-------------------------------------------------|-------------------------------------------------|-------------------------------------------------|-------------------------------------------------|
|                                             |           |              |                   | $T = 1 \times 10^8 \text{ K}$                   |                                                 | $T = 5 \times 10^8$                             |                                                 |
| Decay                                       | $J_p^\pi$ | $J_d^\pi$    | $Q_n(\text{keV})$ | Bound State                                     | Bound State                                     | Bound State                                     | Bound State                                     |
|                                             |           |              |                   | Decay Contribution (%) in Individual Transition | Decay Contribution (%) in Total $\beta^-$ Decay | Decay Contribution (%) in Individual Transition | Decay Contribution (%) in Total $\beta^-$ Decay |
|                                             | $5/2_1^-$ | $3/2_1^-$    | 1494.01           |                                                 |                                                 | 1.72                                            |                                                 |
|                                             |           | $3/2_2^-$    | 1229.35           |                                                 |                                                 | 2.50                                            |                                                 |
|                                             |           | $5/2_1^-$    | 1214.47           |                                                 |                                                 | 2.55                                            |                                                 |
|                                             |           | $5/2_2^-$    | 921.6             |                                                 |                                                 | 4.17                                            |                                                 |
|                                             |           | $3/2_3^-$    | 876.33            |                                                 |                                                 | 4.55                                            |                                                 |
|                                             |           | $7/2_1^-$    | 672.39            |                                                 |                                                 | 6.96                                            |                                                 |
|                                             |           | $3/2_4^-$    | 628.61            |                                                 |                                                 | 7.70                                            |                                                 |
|                                             |           | $7/2_2^-$    | 450.61            |                                                 |                                                 | 12.33                                           |                                                 |
|                                             |           | $3/2_5^-$    | 430.71            |                                                 |                                                 | 13.09                                           |                                                 |
|                                             |           | $3/2_6^-$    | 419.51            |                                                 |                                                 | 13.54                                           |                                                 |
|                                             |           | $7/2_3^-$    | 397.71            |                                                 |                                                 | 14.50                                           |                                                 |
|                                             |           | $7/2_4^-$    | 393.81            |                                                 |                                                 | 14.68                                           |                                                 |
|                                             |           | $3/2_7^-$    | 290.51            |                                                 |                                                 | 21.10                                           |                                                 |
|                                             |           | $7/2_5^-$    | 184.51            |                                                 |                                                 | 33.50                                           |                                                 |
|                                             |           | $3/2_8^-$    | 144.61            |                                                 |                                                 | 41.37                                           |                                                 |
|                                             |           | $3/2_9^-$    | 123.21            |                                                 |                                                 | 46.87                                           |                                                 |
|                                             |           | $5/2_3^-$    | 73.81             |                                                 |                                                 | 65.07                                           |                                                 |
|                                             |           | $3/2_{10}^-$ | 63.51             |                                                 |                                                 | 70.20                                           |                                                 |
|                                             | $5/2_2^-$ | $3/2_1^-$    | 1634.27           |                                                 |                                                 | 1.44                                            |                                                 |
|                                             |           | $3/2_2^-$    | 1369.61           |                                                 |                                                 | 2.03                                            |                                                 |
|                                             |           | $5/2_1^-$    | 1354.73           |                                                 |                                                 | 2.08                                            |                                                 |
|                                             |           | $5/2_2^-$    | 1061.86           |                                                 |                                                 | 3.26                                            |                                                 |
|                                             |           | $3/2_3^-$    | 1016.59           |                                                 |                                                 | 3.52                                            |                                                 |
|                                             |           | $7/2_1^-$    | 812.65            |                                                 |                                                 | 5.15                                            |                                                 |
|                                             |           | $3/2_4^-$    | 768.87            |                                                 |                                                 | 5.63                                            |                                                 |
|                                             |           | $7/2_2^-$    | 590.87            |                                                 |                                                 | 8.44                                            |                                                 |
|                                             |           | $3/2_5^-$    | 570.97            |                                                 |                                                 | 8.88                                            |                                                 |
|                                             |           | $3/2_6^-$    | 559.77            |                                                 |                                                 | 9.13                                            |                                                 |
|                                             |           | $7/2_3^-$    | 537.97            |                                                 |                                                 | 9.67                                            |                                                 |
|                                             |           | $7/2_4^-$    | 534.07            |                                                 |                                                 | 9.77                                            |                                                 |
|                                             |           | $3/2_7^-$    | 430.77            |                                                 |                                                 | 13.09                                           |                                                 |
|                                             |           | $7/2_5^-$    | 324.77            |                                                 |                                                 | 18.57                                           |                                                 |
|                                             |           | $3/2_8^-$    | 284.87            |                                                 |                                                 | 21.56                                           |                                                 |
|                                             |           | $3/2_9^-$    | 263.47            |                                                 |                                                 | 23.49                                           |                                                 |
|                                             |           | $5/2_3^-$    | 214.07            |                                                 |                                                 | 29.08                                           |                                                 |
|                                             |           | $3/2_{10}^-$ | 203.77            |                                                 |                                                 | 30.51                                           |                                                 |
|                                             |           | $3/2_{11}^-$ | 27.97             |                                                 |                                                 | 91.66                                           |                                                 |
| $^{81}\text{Se} \rightarrow ^{81}\text{Br}$ | $1/2_1^-$ | $3/2_1^-$    | 1585.3            | 1.75                                            | 1.81                                            | 1.75                                            | 1.82                                            |
|                                             |           | $1/2_1^-$    | 1047.1            | 3.82                                            |                                                 | 3.81                                            |                                                 |
|                                             |           | $3/2_2^-$    | 1019.26           | 4.01                                            |                                                 | 3.99                                            |                                                 |
|                                             |           | $3/2_3^-$    | 935.4             | 4.64                                            |                                                 | 4.63                                            |                                                 |
|                                             |           | $3/2_4^-$    | 757.01            | 6.57                                            |                                                 | 6.55                                            |                                                 |
|                                             |           | $1/2_2^-$    | 480               | 12.80                                           |                                                 | 12.71                                           |                                                 |
|                                             |           | $3/2_5^-$    | 318.9             | 21.27                                           |                                                 | 21.07                                           |                                                 |
|                                             |           | $3/2_6^-$    | 49.4              | 82.77                                           |                                                 | 81.18                                           |                                                 |
|                                             |           | $3/2_7^-$    | 42.1              | 86.86                                           |                                                 | 85.34                                           |                                                 |
|                                             | $7/2_1^+$ | $9/2_1^+$    | 1152.1            | 3.22                                            |                                                 | 3.21                                            |                                                 |
|                                             |           | $7/2_1^+$    | 316.8             | 21.43                                           |                                                 | 21.23                                           |                                                 |
|                                             |           | $9/2_2^+$    | 146.7             | 45.08                                           |                                                 | 44.30                                           |                                                 |

Table (III.A) continued.

| Transition Details |           |              |                   | $n_e = 1 \times 10^{27} / \text{cm}^3$          |                                                 |                                                 |                                                 |
|--------------------|-----------|--------------|-------------------|-------------------------------------------------|-------------------------------------------------|-------------------------------------------------|-------------------------------------------------|
|                    |           |              |                   | T = $1 \times 10^8$ K                           |                                                 | T = $5 \times 10^8$                             |                                                 |
| Decay              | $J_p^\pi$ | $J_d^\pi$    | $Q_n(\text{keV})$ | Bound State                                     | Bound State                                     | Bound State                                     | Bound State                                     |
|                    |           |              |                   | Decay Contribution (%) in Individual Transition | Decay Contribution (%) in Total $\beta^-$ Decay | Decay Contribution (%) in Individual Transition | Decay Contribution (%) in Total $\beta^-$ Decay |
|                    | $9/2_1^+$ | $9/2_1^+$    | 1343.4            |                                                 |                                                 | 2.42                                            |                                                 |
|                    |           | $7/2_1^+$    | 508.1             |                                                 |                                                 | 11.77                                           |                                                 |
|                    |           | $11/2_1^+$   | 357.3             |                                                 |                                                 | 18.46                                           |                                                 |
|                    |           | $9/2_2^+$    | 338               |                                                 |                                                 | 19.71                                           |                                                 |
|                    |           | $7/2_2^+$    | 90.7              |                                                 |                                                 | 61.48                                           |                                                 |
|                    | $3/2_1^-$ | $3/2_1^-$    | 2053.4            |                                                 |                                                 | 1.03                                            |                                                 |
|                    |           | $5/2_1^-$    | 1777.06           |                                                 |                                                 | 1.39                                            |                                                 |
|                    |           | $1/2_1^-$    | 1514.84           |                                                 |                                                 | 1.92                                            |                                                 |
|                    |           | $3/2_2^-$    | 1487              |                                                 |                                                 | 1.99                                            |                                                 |
|                    |           | $3/2_3^-$    | 1403.14           |                                                 |                                                 | 2.22                                            |                                                 |
|                    |           | $5/2_2^-$    | 1286              |                                                 |                                                 | 2.62                                            |                                                 |
|                    |           | $3/2_4^-$    | 1224.75           |                                                 |                                                 | 2.87                                            |                                                 |
|                    |           | $5/2_3^-$    | 1029.34           |                                                 |                                                 | 3.93                                            |                                                 |
|                    |           | $1/2_2^-$    | 947.74            |                                                 |                                                 | 4.53                                            |                                                 |
|                    |           | $5/2_4^-$    | 863.14            |                                                 |                                                 | 5.30                                            |                                                 |
|                    |           | $3/2_5^-$    | 786.24            |                                                 |                                                 | 6.16                                            |                                                 |
|                    |           | $5/2_5^-$    | 730.04            |                                                 |                                                 | 6.93                                            |                                                 |
|                    |           | $3/2_6^-$    | 540.14            |                                                 |                                                 | 10.82                                           |                                                 |
|                    |           | $3/2_7^-$    | 517.14            |                                                 |                                                 | 11.49                                           |                                                 |
|                    |           | $3/2_8^-$    | 509.84            |                                                 |                                                 | 11.72                                           |                                                 |
|                    |           | $5/2_6^-$    | 254.14            |                                                 |                                                 | 26.93                                           |                                                 |
|                    |           | $3/2_9^-$    | 186.64            |                                                 |                                                 | 36.22                                           |                                                 |
|                    |           | $3/2_{10}^-$ | 167.84            |                                                 |                                                 | 39.71                                           |                                                 |
|                    | $5/2_1^-$ | $3/2_1^-$    | 2076.36           |                                                 |                                                 | 1.02                                            |                                                 |
|                    |           | $5/2_1^-$    | 1800.38           |                                                 |                                                 | 1.38                                            |                                                 |
|                    |           | $3/2_2^-$    | 1510.32           |                                                 |                                                 | 1.97                                            |                                                 |
|                    |           | $3/2_3^-$    | 1426.46           |                                                 |                                                 | 2.20                                            |                                                 |
|                    |           | $5/2_2^-$    | 1309.32           |                                                 |                                                 | 2.59                                            |                                                 |
|                    |           | $3/2_4^-$    | 1248.07           |                                                 |                                                 | 2.83                                            |                                                 |
|                    |           | $7/2_1^-$    | 1239.58           |                                                 |                                                 | 2.87                                            |                                                 |
|                    |           | $5/2_3^-$    | 1052.66           |                                                 |                                                 | 3.86                                            |                                                 |
|                    |           | $5/2_4^-$    | 886.46            |                                                 |                                                 | 5.18                                            |                                                 |
|                    |           | $3/2_5^-$    | 809.56            |                                                 |                                                 | 6.01                                            |                                                 |
|                    |           | $5/2_5^-$    | 753.36            |                                                 |                                                 | 6.74                                            |                                                 |
|                    |           | $7/2_2^-$    | 594.66            |                                                 |                                                 | 9.64                                            |                                                 |
|                    |           | $3/2_6^-$    | 563.46            |                                                 |                                                 | 10.41                                           |                                                 |
|                    |           | $3/2_7^-$    | 540.46            |                                                 |                                                 | 11.04                                           |                                                 |
|                    |           | $3/2_8^-$    | 533.16            |                                                 |                                                 | 11.25                                           |                                                 |
|                    |           | $7/2_3^-$    | 395.16            |                                                 |                                                 | 16.66                                           |                                                 |
|                    |           | $5/2_6^-$    | 277.46            |                                                 |                                                 | 25.01                                           |                                                 |
|                    |           | $3/2_9^-$    | 209.96            |                                                 |                                                 | 33.05                                           |                                                 |
|                    |           | $3/2_{10}^-$ | 191.16            |                                                 |                                                 | 36.01                                           |                                                 |
|                    |           | $7/2_4^-$    | 80.46             |                                                 |                                                 | 66.25                                           |                                                 |
|                    |           | $3/2_{11}^-$ | 20.36             |                                                 |                                                 | 97.14                                           |                                                 |

TABLE (III.B) Variation of bound state  $\beta^-$  decay contribution (in %) for individual transitions and to the total decay with free electron density at a temperature. Column 5 and Column 7: Bound state  $\beta^-$  decay contribution (%) in individual transition. Column 6 and Column 8: contribution (%) to total decay rate from bound state decay. See text for more details.

| Transition Details            |           |           |                   | $T = 3 \times 10^8 K$                                                      |                                                                         |                                                                            |                                                                         |
|-------------------------------|-----------|-----------|-------------------|----------------------------------------------------------------------------|-------------------------------------------------------------------------|----------------------------------------------------------------------------|-------------------------------------------------------------------------|
|                               |           |           |                   | $n_e = 1 \times 10^{26} / cm^3$                                            |                                                                         | $n_e = 1 \times 10^{27} / cm^3$                                            |                                                                         |
| Decay                         | $J_p^\pi$ | $J_d^\pi$ | $Q_n(\text{keV})$ | Bound State<br>Decay<br>Contribution<br>(%) in<br>Individual<br>Transition | Bound State<br>Decay<br>Contribution<br>(%) in Total<br>$\beta^-$ Decay | Bound State<br>Decay<br>Contribution<br>(%) in<br>Individual<br>Transition | Bound State<br>Decay<br>Contribution<br>(%) in Total<br>$\beta^-$ Decay |
| $^{65}Ni \rightarrow ^{65}Cu$ | $5/2_1^-$ | $3/2_1^-$ | 2137.9            | 0.62                                                                       | 1.19                                                                    | 0.60                                                                       | 1.14                                                                    |
|                               |           | $5/2_1^-$ | 1022.3            | 2.68                                                                       |                                                                         | 2.60                                                                       |                                                                         |
|                               |           | $7/2_1^-$ | 656.1             | 5.63                                                                       |                                                                         | 5.48                                                                       |                                                                         |
|                               |           | $5/2_2^-$ | 514.5             | 8.09                                                                       |                                                                         | 7.90                                                                       |                                                                         |
|                               |           | $3/2_2^-$ | 2132.9            | 10.96                                                                      |                                                                         | 10.73                                                                      |                                                                         |
|                               |           | $7/2_2^-$ | 43.56             | 74.52                                                                      |                                                                         | 75.29                                                                      |                                                                         |
|                               |           | $5/2_3^-$ | 30.5              | 84.42                                                                      |                                                                         | 85.35                                                                      |                                                                         |
|                               |           | $1/2_1^-$ | 3/2_1^-           | 2201.27                                                                    |                                                                         | 0.56                                                                       |                                                                         |
|                               |           | $1/2_1^-$ | 1430.63           | 1.42                                                                       |                                                                         | 1.38                                                                       |                                                                         |
|                               |           | $3/2_2^-$ | 476.27            | 9.03                                                                       |                                                                         | 8.82                                                                       |                                                                         |
| $^{66}Cu \rightarrow ^{66}Zn$ | $1_1^+$   | $0_1^+$   | 2640.9            | 0.42                                                                       | 0.61                                                                    | 0.41                                                                       | 0.59                                                                    |
|                               |           | $2_1^+$   | 1601.7            | 1.23                                                                       |                                                                         | 1.19                                                                       |                                                                         |
|                               |           | $2_2^+$   | 768.7             | 4.72                                                                       |                                                                         | 4.59                                                                       |                                                                         |
|                               |           | $0_2^+$   | 269.2             | 19.79                                                                      |                                                                         | 19.49                                                                      |                                                                         |
|                               |           | $2_1^+$   | 1787.65           | 0.98                                                                       |                                                                         | 0.95                                                                       |                                                                         |
|                               | $2_1^+$   | $2_2^+$   | 954.653           | 3.27                                                                       |                                                                         | 3.18                                                                       |                                                                         |
|                               |           | $2_3^+$   | 46.696            | 74.31                                                                      |                                                                         | 75.04                                                                      |                                                                         |
|                               |           | $2_1^+$   | 1876.7            | 0.89                                                                       |                                                                         | 0.86                                                                       |                                                                         |
|                               | $3_1^+$   | $2_2^+$   | 1043.7            | 2.79                                                                       |                                                                         | 2.71                                                                       |                                                                         |
|                               |           | $4_1^+$   | 464.9             | 10.01                                                                      |                                                                         | 9.78                                                                       |                                                                         |
|                               |           | $4_2^+$   | 150.34            | 35.20                                                                      |                                                                         | 35.01                                                                      |                                                                         |
|                               |           | $2_3^+$   | 135.743           | 38.40                                                                      |                                                                         | 38.26                                                                      |                                                                         |

Table (III.B) continued.

| Transition Details                          |           |           |                   | $T = 3 \times 10^8 K$                                                      |                                                                         |                                                                            |                                                                         |
|---------------------------------------------|-----------|-----------|-------------------|----------------------------------------------------------------------------|-------------------------------------------------------------------------|----------------------------------------------------------------------------|-------------------------------------------------------------------------|
|                                             |           |           |                   | $n_e = 1 \times 10^{26} / cm^3$                                            |                                                                         | $n_e = 1 \times 10^{27} / cm^3$                                            |                                                                         |
| Decay                                       | $J_p^\pi$ | $J_d^\pi$ | $Q_n(\text{keV})$ | Bound State<br>Decay<br>Contribution<br>(%) in<br>Individual<br>Transition | Bound State<br>Decay<br>Contribution<br>(%) in Total<br>$\beta^-$ Decay | Bound State<br>Decay<br>Contribution<br>(%) in<br>Individual<br>Transition | Bound State<br>Decay<br>Contribution<br>(%) in Total<br>$\beta^-$ Decay |
| $^{75}\text{Ge} \rightarrow ^{75}\text{As}$ | $1/2_1^-$ | $3/2_1^-$ | 1177.2            | 2.79                                                                       | 3.22                                                                    | 2.71                                                                       | 3.12                                                                    |
|                                             |           | $1/2_1^-$ | 978.594           | 3.88                                                                       |                                                                         | 3.77                                                                       |                                                                         |
|                                             |           | $3/2_2^-$ | 912.542           | 4.37                                                                       |                                                                         | 4.25                                                                       |                                                                         |
|                                             |           | $1/2_2^-$ | 708.46            | 6.59                                                                       |                                                                         | 6.42                                                                       |                                                                         |
|                                             |           | $1/2_3^-$ | 592.2             | 8.64                                                                       |                                                                         | 8.43                                                                       |                                                                         |
|                                             |           | $3/2_3^-$ | 559.52            | 9.37                                                                       |                                                                         | 9.15                                                                       |                                                                         |
|                                             |           | $3/2_4^-$ | 311.8             | 19.83                                                                      |                                                                         | 19.52                                                                      |                                                                         |
|                                             |           | $3/2_5^-$ | 113.9             | 49.81                                                                      |                                                                         | 49.90                                                                      |                                                                         |
|                                             |           | $3/2_6^-$ | 102.7             | 53.43                                                                      |                                                                         | 53.61                                                                      |                                                                         |
|                                             |           | $1/2_4^-$ | 50.2              | 77.25                                                                      |                                                                         | 78.06                                                                      |                                                                         |
|                                             |           | $1/2_5^-$ | 5.2               | 100.00                                                                     |                                                                         | 100.00                                                                     |                                                                         |
|                                             | $7/2_1^+$ | $9/2_1^+$ | 1012.97           | 3.65                                                                       |                                                                         | 3.55                                                                       |                                                                         |
|                                             |           | $5/2_1^+$ | 916.232           | 4.34                                                                       |                                                                         | 4.22                                                                       |                                                                         |
|                                             |           | $5/2_2^+$ | 236.09            | 26.75                                                                      |                                                                         | 26.45                                                                      |                                                                         |
|                                             |           | $5/2_3^+$ | 216.69            | 29.12                                                                      |                                                                         | 28.84                                                                      |                                                                         |
|                                             |           | $9/2_2^+$ | 55.88             | 74.02                                                                      |                                                                         | 74.75                                                                      |                                                                         |
|                                             |           | $5/2_4^+$ | 14.59             | 98.26                                                                      |                                                                         | 98.76                                                                      |                                                                         |
|                                             | $5/2_1^+$ | $5/2_1^+$ | 968.732           | 3.95                                                                       |                                                                         | 3.83                                                                       |                                                                         |
|                                             |           | $5/2_2^+$ | 288.59            | 21.64                                                                      |                                                                         | 21.32                                                                      |                                                                         |
|                                             |           | $5/2_3^+$ | 269.19            | 23.34                                                                      |                                                                         | 23.02                                                                      |                                                                         |
|                                             |           | $5/2_4^+$ | 67.09             | 68.22                                                                      |                                                                         | 68.73                                                                      |                                                                         |
|                                             | $9/2_1^+$ | $9/2_1^+$ | 1073.17           | 3.30                                                                       |                                                                         | 3.20                                                                       |                                                                         |
|                                             |           | $9/2_2^+$ | 116.09            | 49.20                                                                      |                                                                         | 49.22                                                                      |                                                                         |
|                                             | $3/2_1^-$ | $3/2_1^-$ | 1430.35           | 1.93                                                                       |                                                                         | 1.87                                                                       |                                                                         |
|                                             |           | $1/2_1^-$ | 1231.74           | 2.56                                                                       |                                                                         | 2.49                                                                       |                                                                         |
|                                             |           | $3/2_2^-$ | 1165.69           | 2.84                                                                       |                                                                         | 2.76                                                                       |                                                                         |
|                                             |           | $5/2_1^-$ | 1150.81           | 2.91                                                                       |                                                                         | 2.82                                                                       |                                                                         |
|                                             |           | $1/2_2^-$ | 961.61            | 4.00                                                                       |                                                                         | 3.88                                                                       |                                                                         |
|                                             |           | $5/2_2^-$ | 857.94            | 4.85                                                                       |                                                                         | 4.71                                                                       |                                                                         |
|                                             |           | $1/2_3^-$ | 845.35            | 4.97                                                                       |                                                                         | 4.83                                                                       |                                                                         |
|                                             |           | $3/2_3^-$ | 812.67            | 5.30                                                                       |                                                                         | 5.16                                                                       |                                                                         |
|                                             |           | $3/2_4^-$ | 564.95            | 9.24                                                                       |                                                                         | 9.03                                                                       |                                                                         |
|                                             |           | $3/2_5^-$ | 367.05            | 16.36                                                                      |                                                                         | 16.07                                                                      |                                                                         |
|                                             |           | $3/2_6^-$ | 355.85            | 16.99                                                                      |                                                                         | 16.69                                                                      |                                                                         |
|                                             |           | $1/2_4^-$ | 303.35            | 20.46                                                                      |                                                                         | 20.15                                                                      |                                                                         |
|                                             |           | $1/2_5^-$ | 258.35            | 24.37                                                                      |                                                                         | 24.06                                                                      |                                                                         |
|                                             |           | $3/2_7^-$ | 226.85            | 27.84                                                                      |                                                                         | 27.55                                                                      |                                                                         |
|                                             |           | $3/2_8^-$ | 80.95             | 61.76                                                                      |                                                                         | 62.17                                                                      |                                                                         |
|                                             |           | $3/2_9^-$ | 59.55             | 72.02                                                                      |                                                                         | 72.71                                                                      |                                                                         |
|                                             |           | $5/2_3^-$ | 10.15             | 99.57                                                                      |                                                                         | 99.79                                                                      |                                                                         |

Table (III.B) continued.

| Transition Details                          |           |              |                   | $T = 3 \times 10^8 K$                                                      |                                                                     |                                                                            |                                                                     |
|---------------------------------------------|-----------|--------------|-------------------|----------------------------------------------------------------------------|---------------------------------------------------------------------|----------------------------------------------------------------------------|---------------------------------------------------------------------|
|                                             |           |              |                   | $n_e = 1 \times 10^{26} / cm^3$                                            |                                                                     | $n_e = 1 \times 10^{27} / cm^3$                                            |                                                                     |
| Decay                                       | $J_p^\pi$ | $J_d^\pi$    | $Q_n(\text{keV})$ | Bound State<br>Decay<br>Contribution<br>(%) in<br>Individual<br>Transition | Bound State<br>Decay<br>Contribution<br>in Total $\beta^-$<br>Decay | Bound State<br>Decay<br>Contribution<br>(%) in<br>Individual<br>Transition | Bound State<br>Decay<br>Contribution<br>in Total $\beta^-$<br>Decay |
|                                             | $5/2_1^-$ | $3/2_1^-$    | 1494.01           | 1.77                                                                       |                                                                     | 1.72                                                                       |                                                                     |
|                                             |           | $3/2_2^-$    | 1229.35           | 2.57                                                                       |                                                                     | 2.50                                                                       |                                                                     |
|                                             |           | $5/2_1^-$    | 1214.47           | 2.63                                                                       |                                                                     | 2.55                                                                       |                                                                     |
|                                             |           | $5/2_2^-$    | 921.6             | 4.30                                                                       |                                                                     | 4.18                                                                       |                                                                     |
|                                             |           | $3/2_3^-$    | 876.33            | 4.68                                                                       |                                                                     | 4.55                                                                       |                                                                     |
|                                             |           | $7/2_1^-$    | 672.39            | 7.15                                                                       |                                                                     | 6.96                                                                       |                                                                     |
|                                             |           | $3/2_4^-$    | 628.61            | 7.91                                                                       |                                                                     | 7.71                                                                       |                                                                     |
|                                             |           | $7/2_2^-$    | 450.61            | 12.62                                                                      |                                                                     | 12.35                                                                      |                                                                     |
|                                             |           | $3/2_5^-$    | 430.71            | 13.39                                                                      |                                                                     | 13.11                                                                      |                                                                     |
|                                             |           | $3/2_6^-$    | 419.51            | 13.85                                                                      |                                                                     | 13.57                                                                      |                                                                     |
|                                             |           | $7/2_3^-$    | 397.71            | 14.83                                                                      |                                                                     | 14.53                                                                      |                                                                     |
|                                             |           | $7/2_4^-$    | 393.81            | 15.01                                                                      |                                                                     | 14.72                                                                      |                                                                     |
|                                             |           | $3/2_7^-$    | 290.51            | 21.48                                                                      |                                                                     | 21.16                                                                      |                                                                     |
|                                             |           | $7/2_5^-$    | 184.51            | 33.89                                                                      |                                                                     | 33.64                                                                      |                                                                     |
|                                             |           | $3/2_8^-$    | 144.61            | 41.70                                                                      |                                                                     | 41.56                                                                      |                                                                     |
|                                             |           | $7/2_6^-$    | 123.21            | 47.14                                                                      |                                                                     | 47.11                                                                      |                                                                     |
|                                             |           | $3/2_9^-$    | 73.81             | 65.00                                                                      |                                                                     | 65.43                                                                      |                                                                     |
|                                             |           | $3/2_{10}^-$ | 63.51             | 70.03                                                                      |                                                                     | 70.58                                                                      |                                                                     |
| $^{81}\text{Se} \rightarrow ^{81}\text{Br}$ | $1/2_1^-$ | $3/2_1^-$    | 1585.3            | 1.81                                                                       | 1.87                                                                | 1.75                                                                       | 1.81                                                                |
|                                             |           | $1/2_1^-$    | 1047.1            | 3.92                                                                       |                                                                     | 3.81                                                                       |                                                                     |
|                                             |           | $3/2_2^-$    | 1019.26           | 4.11                                                                       |                                                                     | 4.00                                                                       |                                                                     |
|                                             |           | $3/2_3^-$    | 935.4             | 4.77                                                                       |                                                                     | 4.63                                                                       |                                                                     |
|                                             |           | $3/2_4^-$    | 757.01            | 6.73                                                                       |                                                                     | 6.55                                                                       |                                                                     |
|                                             |           | $1/2_2^-$    | 480               | 13.02                                                                      |                                                                     | 12.74                                                                      |                                                                     |
|                                             |           | $3/2_5^-$    | 318.9             | 21.46                                                                      |                                                                     | 21.12                                                                      |                                                                     |
|                                             |           | $3/2_6^-$    | 49.4              | 80.81                                                                      |                                                                     | 81.55                                                                      |                                                                     |
|                                             |           | $3/2_7^-$    | 42.1              | 84.89                                                                      |                                                                     | 85.68                                                                      |                                                                     |
|                                             | $7/2_1^+$ | $9/2_1^+$    | 1152.1            | 3.31                                                                       |                                                                     | 3.21                                                                       |                                                                     |
|                                             |           | $7/2_1^+$    | 316.8             | 21.62                                                                      |                                                                     | 21.28                                                                      |                                                                     |
|                                             |           | $9/2_2^+$    | 146.7             | 44.62                                                                      |                                                                     | 44.51                                                                      |                                                                     |
|                                             | $9/2_1^+$ | $9/2_1^+$    | 1343.4            | 2.49                                                                       |                                                                     | 2.42                                                                       |                                                                     |
|                                             |           | $7/2_1^+$    | 508.1             | 12.06                                                                      |                                                                     | 11.79                                                                      |                                                                     |
|                                             |           | $11/2_1^+$   | 357.3             | 18.83                                                                      |                                                                     | 18.50                                                                      |                                                                     |
|                                             |           | $9/2_2^+$    | 338               | 20.09                                                                      |                                                                     | 19.76                                                                      |                                                                     |
|                                             |           | $7/2_2^+$    | 90.7              | 61.51                                                                      |                                                                     | 61.79                                                                      |                                                                     |

Table (IV) A comparison of terrestrial half-lives ( $T_{1/2(t)}$ ).  $J_p^\pi$  and  $J_d^\pi$  are the spin-parity of the parent and daughter levels, respectively. Experimental  $\beta^-$  branching ( $I_{m(exp)}$ ) from a parent level given in Ref.[4] is normalized to 100%. Theoretical  $\beta^-$  branching ( $I_m$ ) calculations solely take into account  $\beta^-$  decay from the parent levels. Experimental half-lives ( $T_{1/2(t)}$ ) are listed with the error in brackets.

| Decay                                                 | Transition Details [4]               |                             |                      | Shell Model Results          |                       |
|-------------------------------------------------------|--------------------------------------|-----------------------------|----------------------|------------------------------|-----------------------|
|                                                       | $J_p^\pi \rightarrow J_d^\pi$        | Exp. $\beta^-$<br>$I_m(\%)$ | Exp.<br>$T_{1/2(t)}$ | Theo. $\beta^-$<br>$I_m(\%)$ | Theo.<br>$T_{1/2(t)}$ |
| $^{59}\text{Fe} \rightarrow ^{59}\text{Co}$           | $3/2_1^- \rightarrow 3/2_1^-$        | 53.1                        | 44.490 d             | 48.11                        | 41.79 d               |
|                                                       | $3/2_1^- \rightarrow 3/2_2^-$        | 45.3                        |                      | 51.54                        |                       |
|                                                       | $3/2_1^- \rightarrow 1/2_1^-$        | 1.31                        |                      | 0.33                         |                       |
|                                                       | $3/2_1^- \rightarrow 5/2_1^-$        | 0.078                       |                      | 0.02                         |                       |
| $^{61}\text{Co} \rightarrow ^{61}\text{Ni}$           | $7/2_1^- \rightarrow 5/2_1^-$        | 95.6                        | 1.649 hr             | 98.86                        | 1.90 hr               |
|                                                       | $7/2_1^- \rightarrow 5/2_2^-$        | —                           |                      | 0.35                         |                       |
|                                                       | $7/2_1^- \rightarrow 7/2_1^-$        | 4.4                         |                      | 0.50                         |                       |
|                                                       | $7/2_1^- \rightarrow 7/2_2^-$        | —                           |                      | 0.14                         |                       |
|                                                       | $7/2_1^- \rightarrow 5/2_3^-$        | —                           |                      | 0.15                         |                       |
| $^{65}\text{Ni} \rightarrow ^{65}\text{Cu}$           | $5/2_1^- \rightarrow 3/2_1^-$        | 60.0                        | 2.51 hr              | 64.20                        | 2.70 hr               |
|                                                       | $5/2_1^- \rightarrow 5/2_1^-$        | 10.18                       |                      | 5.14                         |                       |
|                                                       | $5/2_1^- \rightarrow 7/2_1^-$        | 28.4                        |                      | 29.44                        |                       |
|                                                       | $5/2_1^- \rightarrow 5/2_2^-$        | 0.89                        |                      | 2.61                         |                       |
|                                                       | $5/2_1^- \rightarrow 3/2_2^-$        | 0.555                       |                      | 0.21                         |                       |
|                                                       | $5/2_1^- \rightarrow 7/2_2^-$        | —                           |                      | 0.01                         |                       |
|                                                       | $5/2_1^- \rightarrow 5/2_3^-$        | —                           |                      | <0.01                        |                       |
| $^{66}\text{Ni} \rightarrow ^{66}\text{Cu}$           | $0_1^+ \rightarrow 1_1^+$            | 100                         | 54.6 hr              | 100                          | 58.98 hr              |
| $^{64}_{29}\text{Cu} \rightarrow ^{64}_{30}\text{Zn}$ | $1_1^+ \rightarrow 0_1^+$            | 100                         | 32.9886 hr           | 100                          | 38.42 hr              |
| $^{66}\text{Cu} \rightarrow ^{66}\text{Zn}$           | $1_1^+ \rightarrow 0_1^+$            | 90.77                       | 5.120 m              | 77.17                        | 7.51 m                |
|                                                       | $1_1^+ \rightarrow 2_1^+$            | 9.01                        |                      | 22.69                        |                       |
|                                                       | $1_1^+ \rightarrow 2_2^+$            | 0.220                       |                      | 0.13                         |                       |
|                                                       | $1_1^+ \rightarrow 0_2^+$            | 0.0037                      |                      | 0.00                         |                       |
| $^{67}\text{Cu} \rightarrow ^{67}\text{Zn}$           | $3/2_1^- \rightarrow 5/2_1^-$        | $\sim 20$                   | 61.83 hr             | 40.64                        | 69.80 hr              |
|                                                       | $3/2_1^- \rightarrow 1/2_1^-$        | $\sim 22$                   |                      | 21.50                        |                       |
|                                                       | $3/2_1^- \rightarrow 3/2_1^-$        | $\sim 57$                   |                      | 35.87                        |                       |
|                                                       | $3/2_1^- \rightarrow 3/2_2^-$        | $\sim 1.1$                  |                      | 1.99                         |                       |
| $^{69}\text{Zn} \rightarrow ^{69}\text{Ga}$           | $1/2_1^- \rightarrow 3/2_1^-$        | 99.9986                     | 56.4 m               | 99.99                        | 54.72 m               |
|                                                       | $1/2_1^- \rightarrow 1/2_1^-$        | 0.0012                      |                      | 0.01                         |                       |
|                                                       | $1/2_1^- \rightarrow 3/2_2^-$        | 0.00025                     |                      | $\sim 0.00$                  |                       |
| $^{72}\text{Zn} \rightarrow ^{72}\text{Ga}$           | $0_1^+ \rightarrow 0_1^+$            | <0.01                       | 46.5 hr              | —                            | 55.54 hr              |
|                                                       | $0_1^+ \rightarrow 1_1^+$            | 0.21                        |                      | —                            |                       |
|                                                       | $0_1^+ \rightarrow 1_2^+$            | 85.1                        |                      | 64.42                        |                       |
|                                                       | $0_1^+ \rightarrow 1_3^+$            | 14.7                        |                      | 35.58                        |                       |
| $^{70}\text{Ga} \rightarrow ^{70}\text{Ge}$           | $1_1^+ \rightarrow 0_1^+$            | 98.91                       | 21.23 m              | 97.02                        | 21.46 m               |
|                                                       | $1_1^+ \rightarrow 2_1^+$            | 0.36                        |                      | 2.62                         |                       |
|                                                       | $1_1^+ \rightarrow 0_2^+$            | 0.32                        |                      | 0.36                         |                       |
| $^{78}\text{Ge} \rightarrow ^{78}\text{As}$           | $0_1^+ \rightarrow 1_1^+$            | 96                          | 88 m                 | 40.64                        | 88.44 m               |
|                                                       | $0_1^+ \rightarrow 1_2^+$            | 4                           |                      | 14.81                        |                       |
|                                                       | $0_1^+ \rightarrow 1_3^+$            | —                           |                      | 44.54                        |                       |
| $^{81}\text{Se} \rightarrow ^{81}\text{Br}$           | $1/2_1^- \rightarrow 3/2_1^-$        | 98.73                       | 18.45 m              | 98.78                        | 19.78 m               |
|                                                       | $1/2_1^- \rightarrow 1/2_1^-$        | 0.034                       |                      | 0.02                         |                       |
|                                                       | $1/2_1^- \rightarrow 3/2_2^-$        | 0.79                        |                      | 0.10                         |                       |
|                                                       | $1/2_1^- \rightarrow 3/2_3^-$        | 0.0196                      |                      | 0.18                         |                       |
|                                                       | $1/2_1^- \rightarrow 3/2_4^-$        | 0.40                        |                      | 0.89                         |                       |
|                                                       | $1/2_1^- \rightarrow 1/2_2^-$        | —                           |                      | 0.03                         |                       |
|                                                       | $1/2_1^- \rightarrow 3/2_5^-$        | —                           |                      | $\sim 0.01$                  |                       |
|                                                       | $1/2_1^- \rightarrow 3/2_6^-$        | —                           |                      | <0.01                        |                       |
|                                                       | $1/2_1^- \rightarrow 3/2_7^-$        | —                           |                      | <0.01                        |                       |
|                                                       | $^{a,b} 7/2_1^+ \rightarrow 9/2_1^+$ | 100                         |                      | 100                          |                       |

Table (V) Total  $\beta^-$  decay rate ( $\lambda_{bare(s)}$ ) and half-life ( $T_{1/2(bare(s))}$ ) of bare atoms in different density - temperature combinations and comparison with previous results (CT [6] and TY [5]). Half-life of a nucleus is given in unit of min/ hr/ d /yr, as the abbreviations of minute/ hour/ day/ year, respectively. Here,  $T_1$  stands for environmental temperature  $T = 1 \times 10^8 K$ ,  $T_3$  for  $T = 3 \times 10^8 K$  and  $T_5$  for  $T = 5 \times 10^8 K$ . R is the ratio of calculated neutral atom terrestrial half-life to bare atom stellar half-life, i.e  $R = T_{1/2(t)}/T_{1/2(bare(s))}$ . See text for details.

| This Work                     |                               |                    |       |                               |                    |       | Previous Results              |                               |
|-------------------------------|-------------------------------|--------------------|-------|-------------------------------|--------------------|-------|-------------------------------|-------------------------------|
| Decay                         | $n_e = 1 \times 10^{26}/cm^3$ |                    |       | $n_e = 1 \times 10^{27}/cm^3$ |                    |       | $n_e = 1 \times 10^{27}/cm^3$ | $n_e = 1 \times 10^{26}/cm^3$ |
|                               | $\lambda_{bare(s)}$           | $T_{1/2(bare(s))}$ | R     | $\lambda_{bare(s)}$           | $T_{1/2(bare(s))}$ | R     | $\lambda_{bare(s)}(CT)$       | $\lambda_{bare(s)}(TY)$       |
| $^{59}Fe \rightarrow ^{59}Co$ | $T_1$ $2.10 \times 10^{-7}$   | 38.11 d            | 1.097 | $2.05 \times 10^{-7}$         | 39.06 d            | 1.070 |                               | $1.80 \times 10^{-7}$         |
|                               | $T_3$ $2.11 \times 10^{-7}$   | 38.01 d            | 1.099 | $2.07 \times 10^{-7}$         | 38.68 d            | 1.080 |                               |                               |
|                               | $T_5$ $2.28 \times 10^{-7}$   | 35.13 d            | 1.190 | $2.25 \times 10^{-7}$         | 35.62 d            | 1.178 |                               | $1.88 \times 10^{-7}$         |
| $^{61}Co \rightarrow ^{61}Ni$ | $T_1$ $1.02 \times 10^{-4}$   | 1.89 hr            | 1.005 | $1.01 \times 10^{-4}$         | 1.90 hr            | 1.000 |                               | $1.17 \times 10^{-4}$         |
|                               | $T_3$ $1.02 \times 10^{-4}$   | 1.89 hr            | 1.005 | $1.02 \times 10^{-4}$         | 1.90 hr            | 1.000 |                               |                               |
|                               | $T_5$ $1.02 \times 10^{-4}$   | 1.89 hr            | 1.005 | $1.02 \times 10^{-4}$         | 1.89 hr            | 1.005 |                               | $1.17 \times 10^{-4}$         |
| $^{65}Ni \rightarrow ^{65}Cu$ | $T_1$ $7.31 \times 10^{-5}$   | 2.63 hr            | 1.027 | $7.26 \times 10^{-5}$         | 2.65 hr            | 1.019 |                               | $7.64 \times 10^{-5}$         |
|                               | $T_3$ $2.20 \times 10^{-4}$   | 52.39 min          | 3.092 | $2.20 \times 10^{-4}$         | 52.56 min          | 3.082 |                               |                               |
|                               | $T_5$ $4.51 \times 10^{-4}$   | 25.63 min          | 6.321 | $4.50 \times 10^{-4}$         | 25.69 min          | 6.308 |                               | $7.72 \times 10^{-5}$         |
| $^{66}Ni \rightarrow ^{66}Cu$ | $T_1$ $3.86 \times 10^{-6}$   | 49.89 hr           | 1.182 | $3.73 \times 10^{-6}$         | 51.64 hr           | 1.142 |                               | $3.51 \times 10^{-6}$         |
|                               | $T_3$ $3.87 \times 10^{-6}$   | 49.71 hr           | 1.186 | $3.78 \times 10^{-6}$         | 50.94 hr           | 1.158 |                               |                               |
|                               | $T_5$ $3.88 \times 10^{-6}$   | 49.64 hr           | 1.188 | $3.80 \times 10^{-6}$         | 50.67 hr           | 1.164 |                               | $3.51 \times 10^{-6}$         |
| $^{64}Cu \rightarrow ^{64}Zn$ | $T_1$ $5.34 \times 10^{-6}$   | 36.05 hr           | 1.066 | $5.25 \times 10^{-6}$         | 36.66 hr           | 1.048 | $1.20 \times 10^{-5}$         | $6.06 \times 10^{-6}$         |
|                               | $T_3$ $5.35 \times 10^{-6}$   | 36.01 hr           | 1.067 | $5.28 \times 10^{-6}$         | 36.45 hr           | 1.054 |                               |                               |
|                               | $T_5$ $5.35 \times 10^{-6}$   | 35.99 hr           | 1.068 | $5.29 \times 10^{-6}$         | 36.36 hr           | 1.057 | $1.30 \times 10^{-5}$         | $5.81 \times 10^{-6}$         |
| $^{66}Cu \rightarrow ^{66}Zn$ | $T_1$ $1.53 \times 10^{-3}$   | 7.54 min           | 0.996 | $1.53 \times 10^{-3}$         | 7.57 min           | 0.992 |                               | $2.27 \times 10^{-3}$         |
|                               | $T_3$ $1.53 \times 10^{-3}$   | 7.55 min           | 0.995 | $1.53 \times 10^{-3}$         | 7.57 min           | 0.992 |                               |                               |
|                               | $T_5$ $1.50 \times 10^{-3}$   | 7.71 min           | 0.974 | $1.50 \times 10^{-3}$         | 7.72 min           | 0.973 |                               | $2.21 \times 10^{-3}$         |
| $^{67}Cu \rightarrow ^{67}Zn$ | $T_1$ $2.98 \times 10^{-6}$   | 64.50 hr           | 1.084 | $2.92 \times 10^{-6}$         | 65.81 hr           | 1.061 |                               | $3.11 \times 10^{-6}$         |
|                               | $T_3$ $2.99 \times 10^{-6}$   | 64.35 hr           | 1.084 | $2.95 \times 10^{-6}$         | 65.30 hr           | 1.069 |                               |                               |
|                               | $T_5$ $2.99 \times 10^{-6}$   | 64.30 hr           | 1.084 | $2.96 \times 10^{-6}$         | 65.10 hr           | 1.072 |                               | $3.11 \times 10^{-6}$         |
| $^{69}Zn \rightarrow ^{69}Ga$ | $T_1$ $2.15 \times 10^{-4}$   | 53.64 min          | 1.020 | $2.13 \times 10^{-4}$         | 54.15 min          | 1.011 |                               | $2.06 \times 10^{-4}$         |
|                               | $T_3$ $2.15 \times 10^{-4}$   | 53.57 min          | 1.021 | $2.14 \times 10^{-4}$         | 53.94 min          | 1.014 |                               |                               |
|                               | $T_5$ $2.16 \times 10^{-4}$   | 53.55 min          | 1.021 | $2.14 \times 10^{-4}$         | 53.87 min          | 1.016 |                               | $2.06 \times 10^{-4}$         |
| $^{72}Zn \rightarrow ^{72}Ga$ | $T_1$ $6.71 \times 10^{-6}$   | 28.69 hr           | 1.936 | $6.50 \times 10^{-6}$         | 29.64 hr           | 1.874 |                               | $4.14 \times 10^{-6}$         |
|                               | $T_3$ $6.73 \times 10^{-6}$   | 28.59 hr           | 1.943 | $6.58 \times 10^{-6}$         | 29.27 hr           | 1.898 |                               |                               |
|                               | $T_5$ $6.74 \times 10^{-6}$   | 28.56 hr           | 1.945 | $6.61 \times 10^{-6}$         | 29.13 hr           | 1.907 |                               | $4.14 \times 10^{-6}$         |
| $^{70}Ga \rightarrow ^{70}Ge$ | $T_1$ $5.40 \times 10^{-4}$   | 21.39 min          | 1.003 | $5.37 \times 10^{-4}$         | 21.49 min          | 0.999 |                               | $5.46 \times 10^{-4}$         |
|                               | $T_3$ $5.40 \times 10^{-4}$   | 21.37 min          | 1.004 | $5.38 \times 10^{-4}$         | 21.45 min          | 1.001 |                               |                               |
|                               | $T_5$ $5.41 \times 10^{-4}$   | 21.37 min          | 1.004 | $5.39 \times 10^{-4}$         | 21.44 min          | 1.001 |                               | $5.46 \times 10^{-4}$         |
| $^{78}Ge \rightarrow ^{78}As$ | $T_1$ $1.41 \times 10^{-4}$   | 1.36 hr            | 1.084 | $1.38 \times 10^{-4}$         | 1.39 hr            | 1.060 |                               | $1.33 \times 10^{-4}$         |
|                               | $T_3$ $1.41 \times 10^{-4}$   | 1.36 hr            | 1.084 | $1.39 \times 10^{-4}$         | 1.38 hr            | 1.068 |                               |                               |
|                               | $T_5$ $1.41 \times 10^{-4}$   | 1.36 hr            | 1.084 | $1.40 \times 10^{-4}$         | 1.38 hr            | 1.068 |                               | $1.33 \times 10^{-4}$         |
| $^{81}Se \rightarrow ^{81}Br$ | $T_1$ $5.86 \times 10^{-4}$   | 19.71 min          | 1.004 | $5.83 \times 10^{-4}$         | 19.82 min          | 0.998 |                               | $6.24 \times 10^{-4}$         |
|                               | $T_3$ $5.46 \times 10^{-4}$   | 21.16 min          | 0.935 | $5.44 \times 10^{-4}$         | 21.24 min          | 0.931 |                               |                               |
|                               | $T_5$ $4.28 \times 10^{-4}$   | 26.97 min          | 0.733 | $4.27 \times 10^{-4}$         | 27.08 min          | 0.730 |                               | $4.57 \times 10^{-4}$         |

In case of  $^{81}Se$  the value of R is determined taking the contribution of ground state terrestrial half-life only.
